# Supplementary material for: Skin Lesion Phenotyping via Nested Multi-modal Contrastive Learning
Source: arXiv:2505.23709 source file (2026-01-22)
Supplement: Supplementary file 1 [file 1_vit_back.tex]

showcasing the benefit of higher-capacity models for feature extraction. Interestingly, for our datasets, the differences between encoder sizes are less pronounced, suggesting that the task complexity or data distribution may not fully leverage the increased capacity of larger encoders.

In comparison to linear probing and k-NN approaches, these results highlight a divergence, as the latter often fail to exhibit consistent performance gains with larger encoder sizes. This difference can be attributed to the improved optimization and fine-tuning capabilities of the proposed method, which allow it to better exploit the representational capacity of larger ViTs. Table~\ref{tab:params} further highlights the significant difference in parameter counts across encoder sizes, with ViT-Base being over 4x larger than ViT-Small and over 15x larger than ViT-Tiny.

Additionally, the choice of N, the number of images and lesions selected per patient during training, also plays a role in performance differences. For ViT-Tiny and ViT-Small, N=100 was chosen to balance computation and training efficiency, while for ViT-Base, N=50 was used due to the model's significantly larger size and computational requirements. This reduction in N for ViT-Base could partially explain the performance drop observed in certain datasets, as the model has less diverse data per patient for training.

Notably, ViT-Small tends to strike the best balance between performance and model complexity, as seen across most datasets. Given its favorable trade-off, this is the configuration adopted in the main paper, while this analysis is provided as supplementary material to highlight the broader implications of encoder size and training setup.

SECTION?

This analysis compares the performance of SLIMP-C using two tabular encoders: FT-Transformer (\cite{ref}) and TRACE (\cite{ref}). The results in Table~\ref{tab:tabular_encoders} show their performance across PAD-UFES-20, HIBA, and HAM10000, using the ViT-Small image encoder.

TRACE, which is specifically designed for medical data, consistently performs better than the more general FT-Transformer across all datasets and metrics, including Accuracy (Acc), Balanced Accuracy (BAcc), F1 Score, and Area Under the ROC Curve (Auroc Curve). This highlights how a specialized design like TRACE can better handle the nuances of medical tabular data.

Interestingly, FT-Transformer is much larger, with 178.4 million parameters compared to TRACE’s 42.5 million. Despite being over four times bigger, FT-Transformer doesn’t achieve the same level of performance. This shows that simply having a larger model isn’t enough—TRACE’s task-specific design allows it to make better use of the data.

Overall, TRACE offers a strong balance of efficiency and performance, making it the better choice for SLIMP-C when working with medical data.

\begin{table}[htbp]
\centering
\resizebox{\columnwidth}{!}{
      \begin{tabular}{cccccc}
      &       & \multicolumn{4}{c}{\textbf{PAD-UFES-20}} \\
      &       & Acc   & BAcc  & F1    & Auroc Curve \\ 
      \hline
      \multirow{6}[2]{*}{\begin{sideways}linprob\end{sideways}} & SLIMP-C w/ $P=4$  & \textbf{90.0}  & 86.4  & 0.886 & 0.907 \\
      & SLIMP-C w/ $P=8$   & 89.1 & 88.4 & 0.906 & 0.911 \\
      & SLIMP-C w/ $P=32$  & 88.7 & 88.4 & 0.898 & \textbf{0.928} \\
      & \cellcolor{lightblue} SLIMP-C w/ $P=64$  & \cellcolor{lightblue} \textbf{90.0} & \cellcolor{lightblue} \textbf{89.5} & \cellcolor{lightblue} \textbf{0.913} & \cellcolor{lightblue} 0.917 \\
      & SLIMP-C w/ $P=128$ & 89.6 & 89.1 & 0.908 & 0.918 \\
      & SLIMP-C w/ $P=256$ & 89.6 & 89.1 & 0.908 & 0.927 \\
      \bottomrule
      \end{tabular}%
      }
      \caption{...}\label{tab:slimpc-b}%
\end{table}%

  % Table generated by Excel2LaTeX from sheet 'Supplementary'
  \begin{table}[htbp]
    \centering
      \begin{tabular}{c|ccc}
            & \multicolumn{3}{c}{\textbf{SLIMP-C \# of parameters (milions)}} \\
      \multicolumn{1}{c|}{\textbf{Dataset}} & ViT-Tiny & ViT-Small & ViT-Base \\\hline
      HAM1000 & 10.8  & 42.3  & 167.3 \\
      HIBA  & 10.8  & 42.3  & 167.3 \\
      PAD-UFES-20 & 10.9  & 42.6  & 168.6 \\
      PH2   & 9.8   & 38.5  & 152.0 \\
      \end{tabular}%
      \caption{Number of parameters calculated cumulatively for SLIMP and SLIMP-C pipeline for different choices of image encoders.}\label{tab:params}%
\end{table}%

\begin{table*}[b!]
    \centering
    \resizebox{\textwidth}{!}{
      \begin{tabular}{cccccc|cccc|cccc|cccc}
            &       & \multicolumn{4}{c}{\textbf{PAD-UFES-20}} & \multicolumn{4}{c}{\textbf{HIBA}} & \multicolumn{4}{c}{\textbf{HAM10000}} & \multicolumn{4}{c}{\textbf{PH2 - image +lesion}} \\
            &       & Acc   & BAcc  & F1    & Auroc Curve & Acc   & BAcc  & F1    & Auroc Curve & Acc   & BAcc  & F1    & Auroc Curve & Acc   & BAcc  & F1    & Auroc Curve \\\hline
      \multirow{3}[2]{*}{\begin{sideways}linprob\end{sideways}} & SLIMP-C w/ ViT-Tiny & 89.6  & 89.0  & 0.908 & 0.922 & 87.7  & 89.5  & 0.884 & 0.944 & 85.7  & 74.0  & 0.602 & 0.905 & \textbf{95.0} & 91.7  & 0.909 & \textbf{1.000} \\
            & SLIMP-C w/ ViT-Small & \textbf{90.0} & \textbf{89.5} & \textbf{0.913} & 0.917 & \textbf{90.7} & \textbf{90.7} & \textbf{0.912} & \textbf{0.944} & \textbf{86.8} & \textbf{82.7} & \textbf{0.694} & \textbf{0.922} & \textbf{95.0} & \textbf{96.4} & \textbf{0.923} & 0.988 \\
            & SLIMP-C w/ ViT-Base & 87.8  & 87.5  & 0.892 & \textbf{0.931} & 89.5  & 89.4  & 0.901 & 0.942 & 85.2  & 73.7  & 0.593 & 0.905 & 90.0  & 83.3  & 0.800 & \textbf{1.000} \\
      \hline
      \multirow{3}[2]{*}{\begin{sideways}kNN\end{sideways}} & SLIMP-C w/ ViT-Tiny & 81.7  & 81.4  & 0.837 & 0.858 & 79.6  & 79.5  & \textbf{0.807} & 0.887 & 85.6  & \textbf{74.3} & \textbf{0.604} & 0.890 & 90.0  & 83.3  & 0.800 & \textbf{1.000} \\
            & SLIMP-C w/ ViT-Small & 82.2  & 81.4  & 0.846 & 0.883 & \textbf{80.3} & \textbf{80.4} & 0.800 & \textbf{0.897} & \textbf{86.1} & 73.7  & 0.602 & \textbf{0.897} & \textbf{95.0} & \textbf{96.4} & \textbf{0.923} & 0.988 \\
            & SLIMP-C w/ ViT-Base & \textbf{84.4} & \textbf{84.0} & \textbf{0.861} & \textbf{0.896} & 80.3  & 80.5  & 0.798 & 0.892 & 83.4  & 71.2  & 0.549 & 0.870 & 80.0  & 66.7  & 0.500 & \textbf{1.000} \\
      \bottomrule
      \end{tabular}%
      }
      \caption{Impact of image encoder size on the skin classification performance using SLIMP-C.}\label{tab:vitsize}%
  \end{table*}%
