# Supplementary material for: Skin Lesion Phenotyping via Nested Multi-modal Contrastive Learning
Source: arXiv:2505.23709 source file (2026-01-22)
Supplement: Supplementary file 2 [file 4_attmaps_tab.tex]

By utilizing TRACE to encode the tabular metadata, we exploit the self-attention mechanism, to gain valuable insights about the decision-making process during the downstream task, as visualized by the feature attention maps in Figures \ref{fig:isic_attention_maps}, \ref{fig:padufes20_attention_maps}, \ref{fig:ham10000_attention_maps}, \ref{fig:hiba_attention_maps}, \ref{fig:ph2_attention_maps} for each target dataset.

More specifically, Figure 2 represents the attention weight visualizations for the melanoma (left) and heart disease/attack (right) classification tasks. Its aim is to identify the features that predominantly influence the final positive diagnosis. Rows represent participants randomly selected from the validation set and columns the key features considered during training. Each cell is calculated by averaging the attention weights of each key feature across all input queries. For instance, the frequency of skin checks a patient has, consistently provides high attention weights across the majority of the participants within the melanoma dataset.

\begin{figure}[htb]
    \centering
    \begin{tabular}{c} % First row: single centered figure
        Clinical Features \\ % Caption for the first figure
        \includegraphics[width=0.5\textwidth]{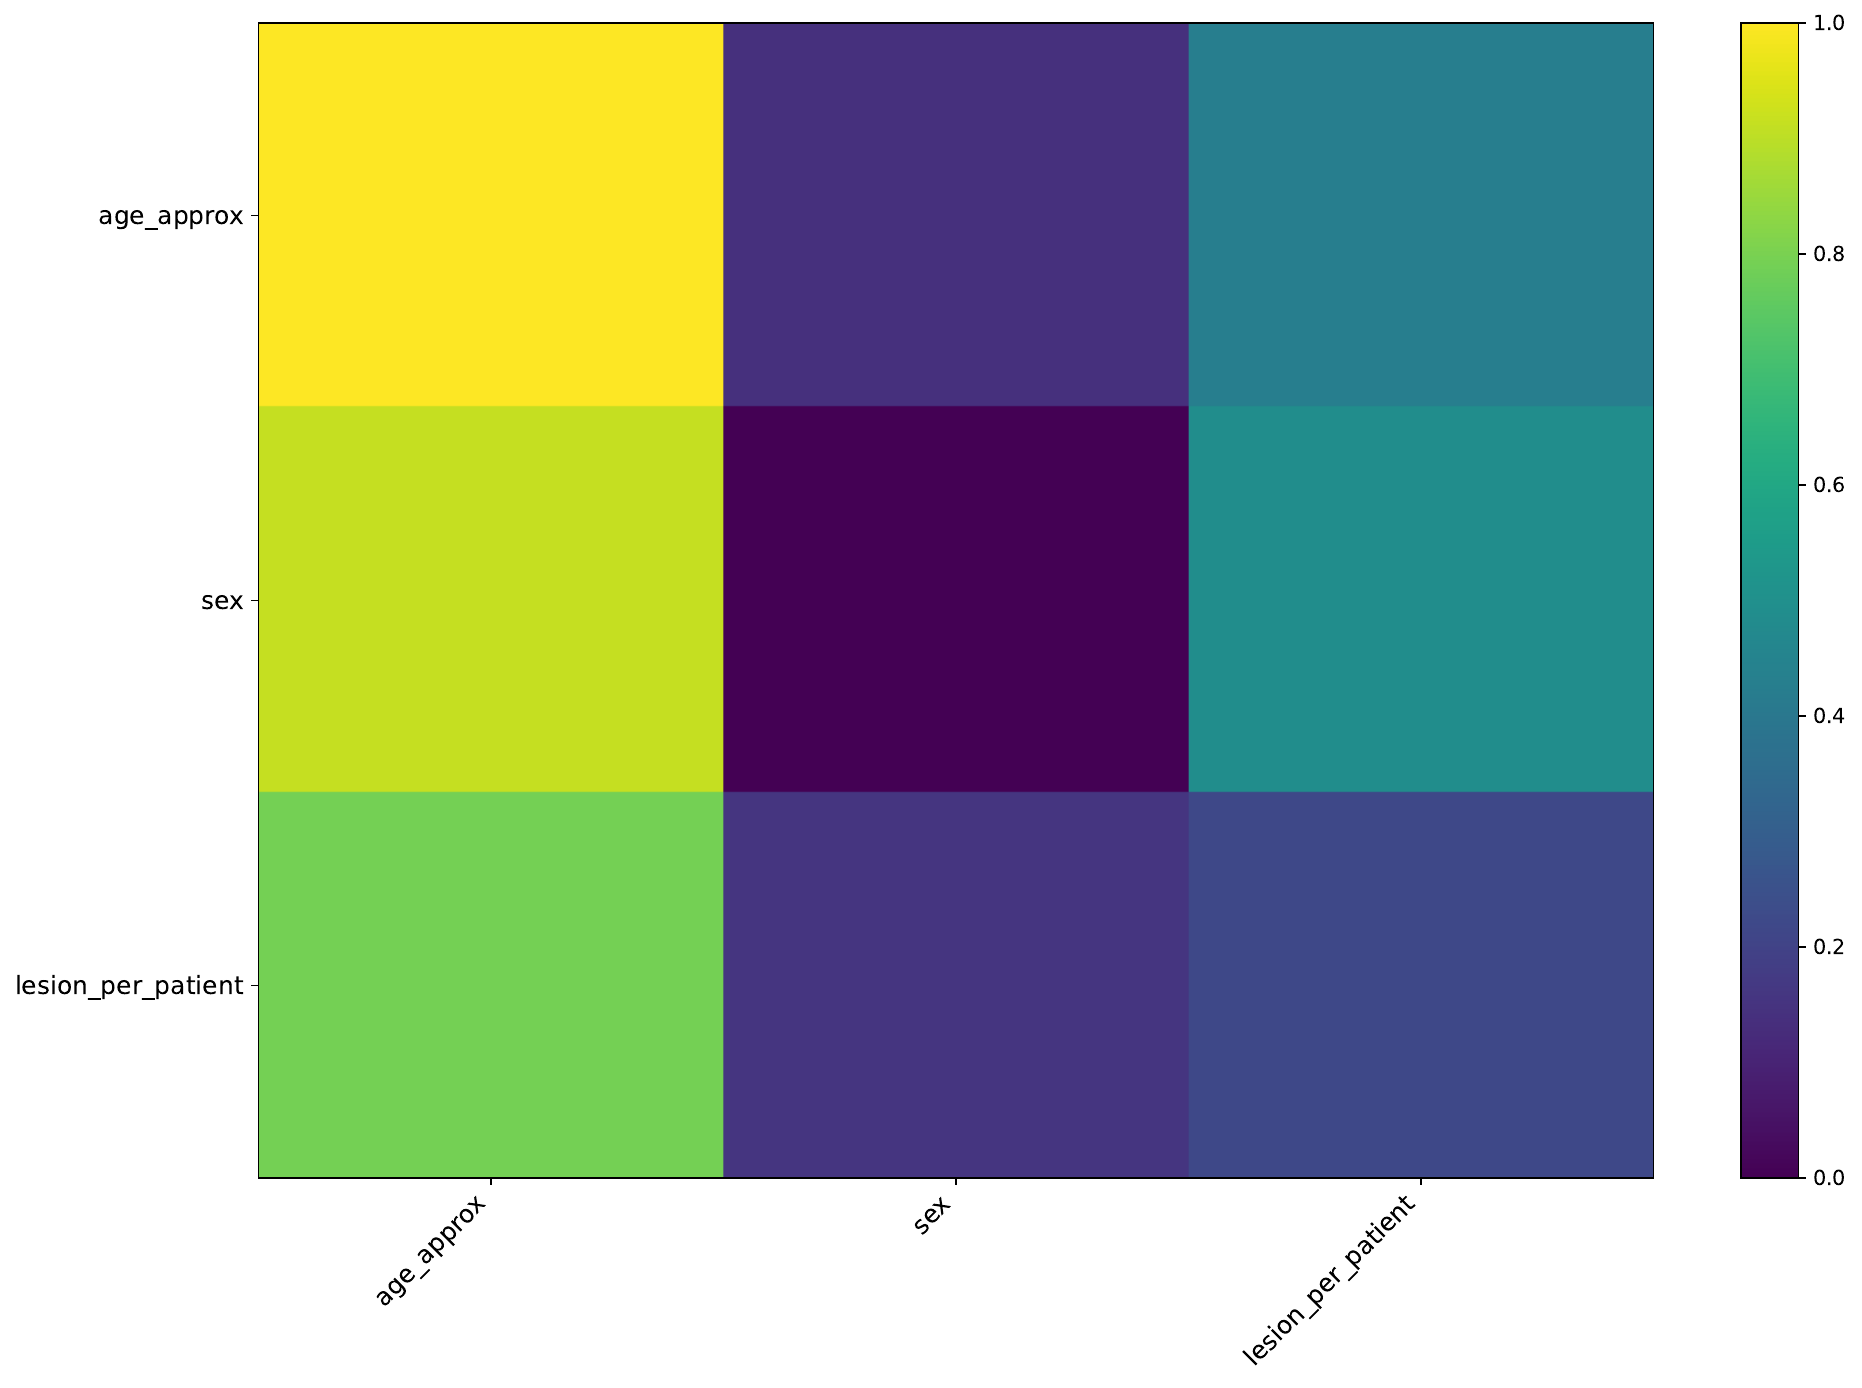} \\
    \end{tabular}

    \vspace{1em} % Vertical space between rows

    \begin{tabular}{cc} % Second row: two figures side-by-side
        Benign Lesion Features & Malignant Lesion Features \\ % Captions for the second row
        \includegraphics[width=0.5\textwidth]{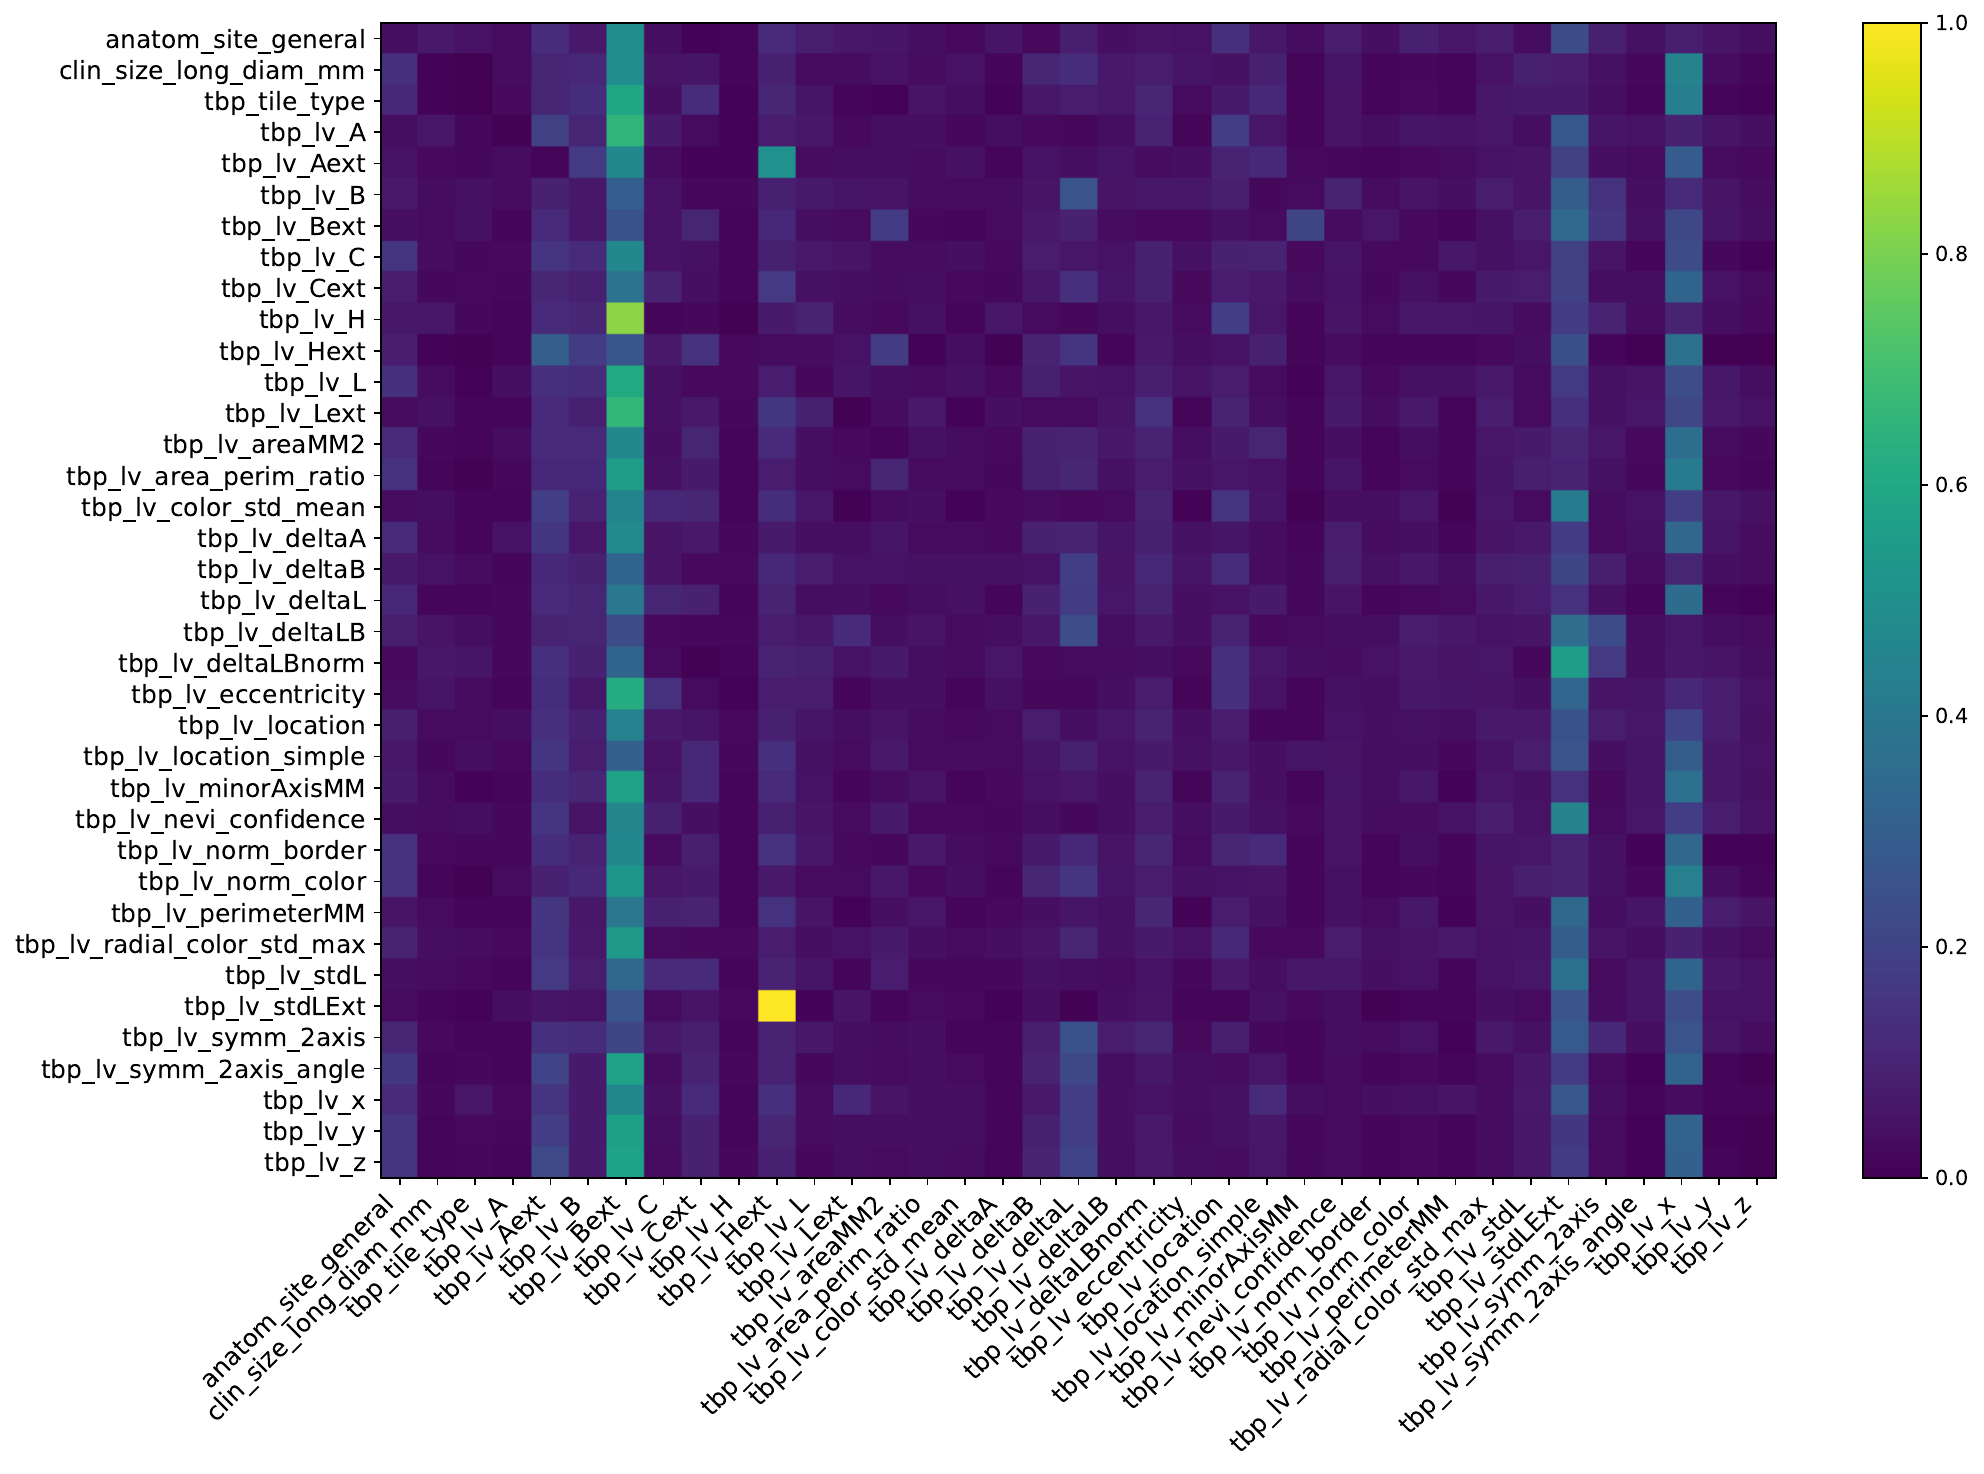} &
        \includegraphics[width=0.5\textwidth]{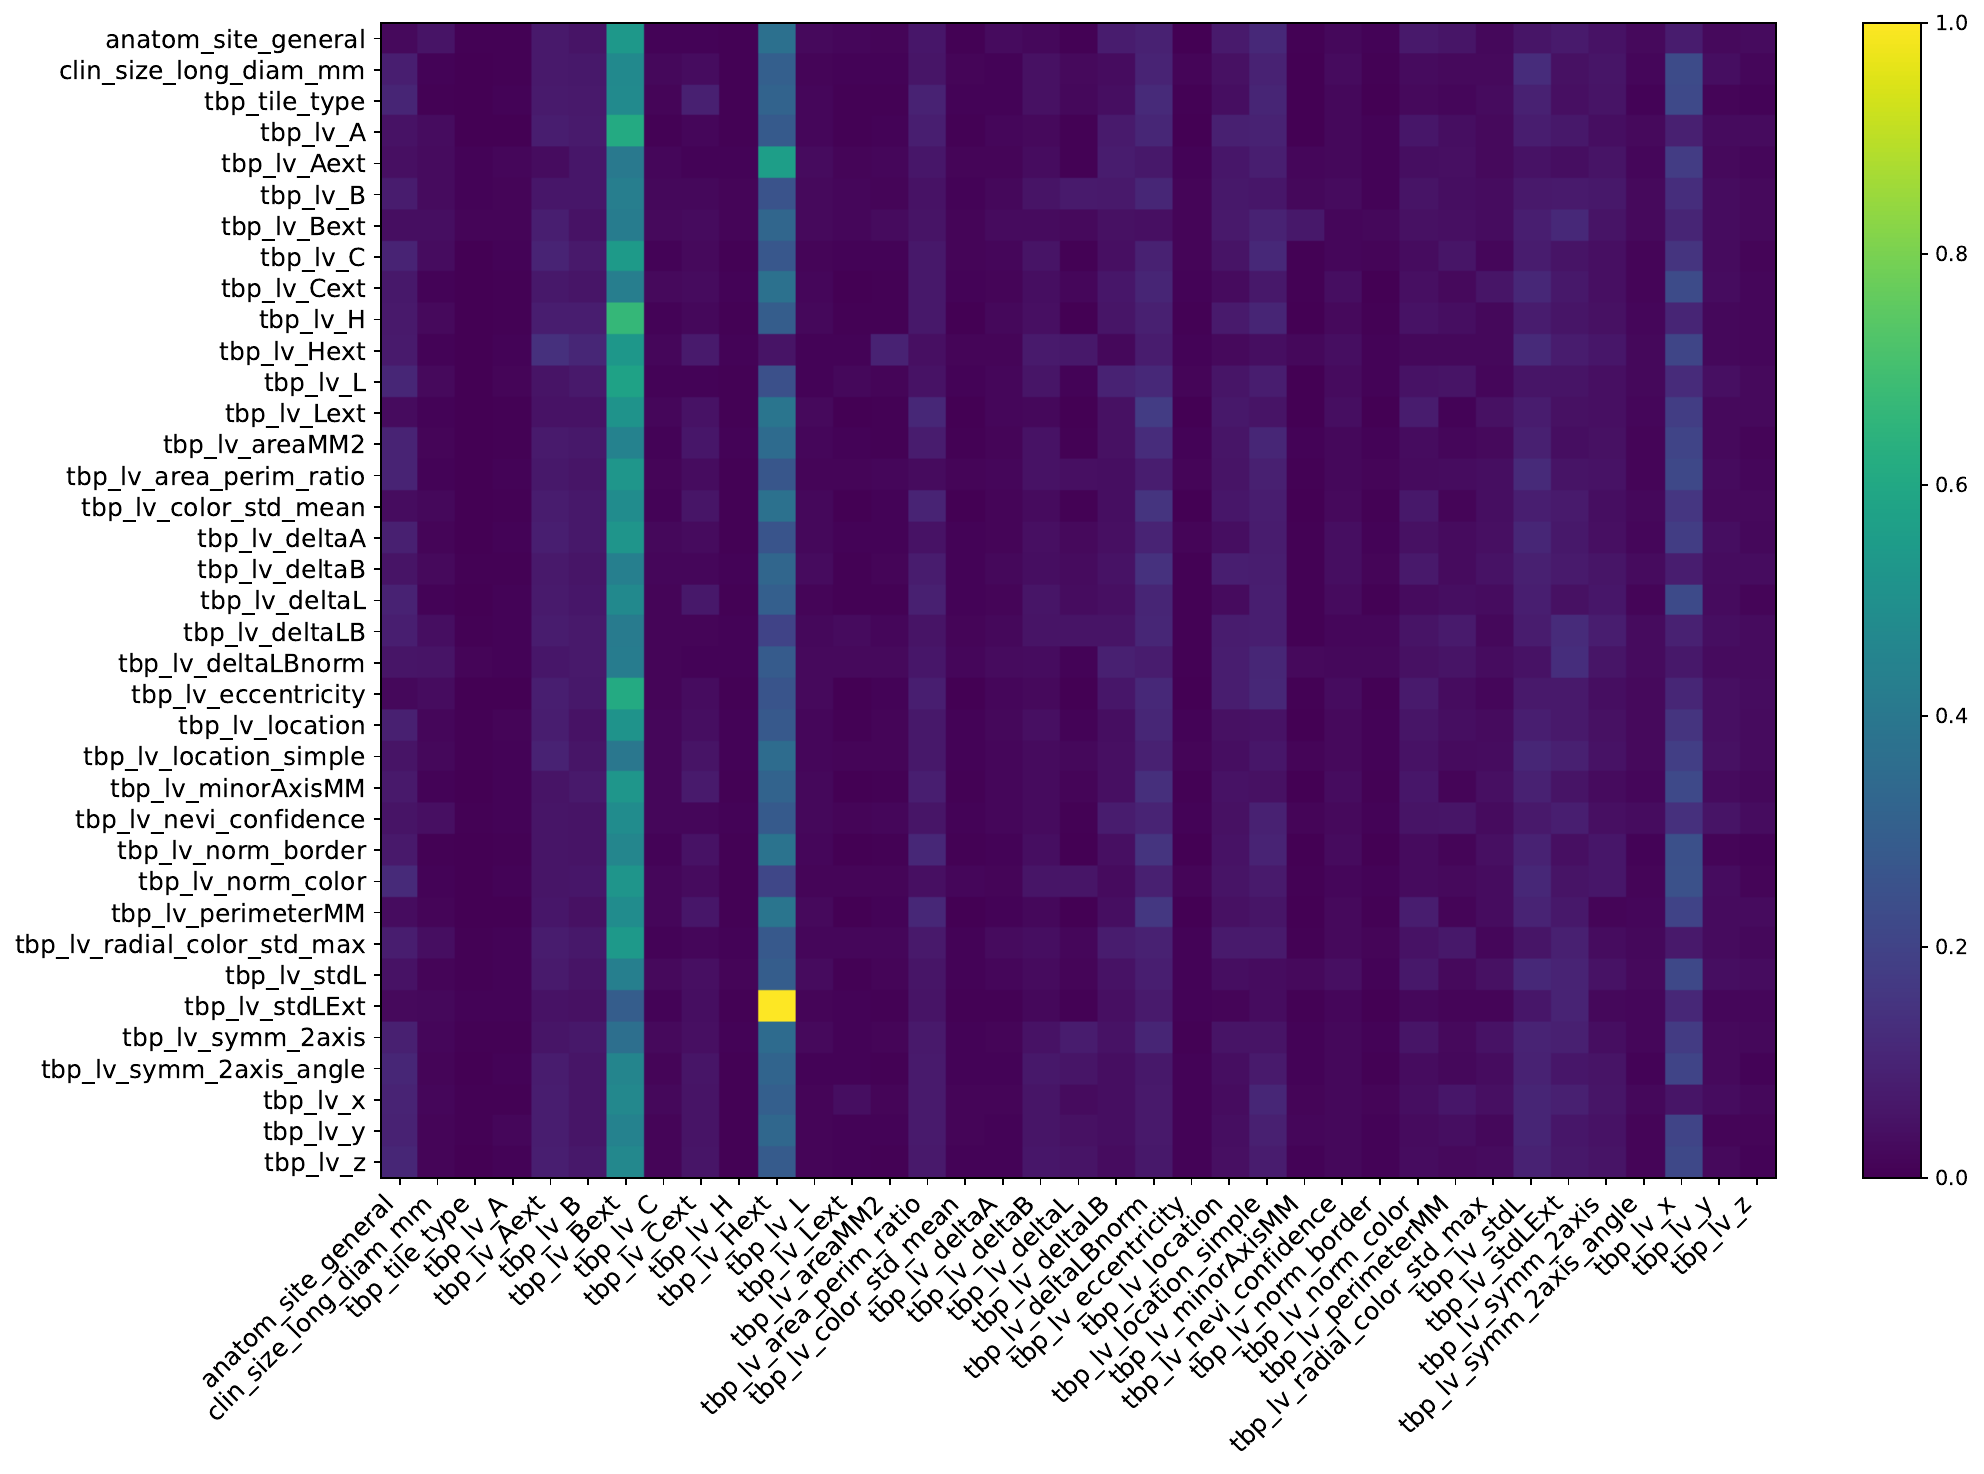} \\
    \end{tabular}

    \caption{Attention maps for the SLICE-3D dataset.}
    \label{fig:isic_attention_maps}
\end{figure}

\begin{figure}[htb]
    \centering
    \begin{tabular}{c} % First row: single centered figure
        Clinical Features \\ % Caption for the first figure
        \includegraphics[width=0.5\textwidth]{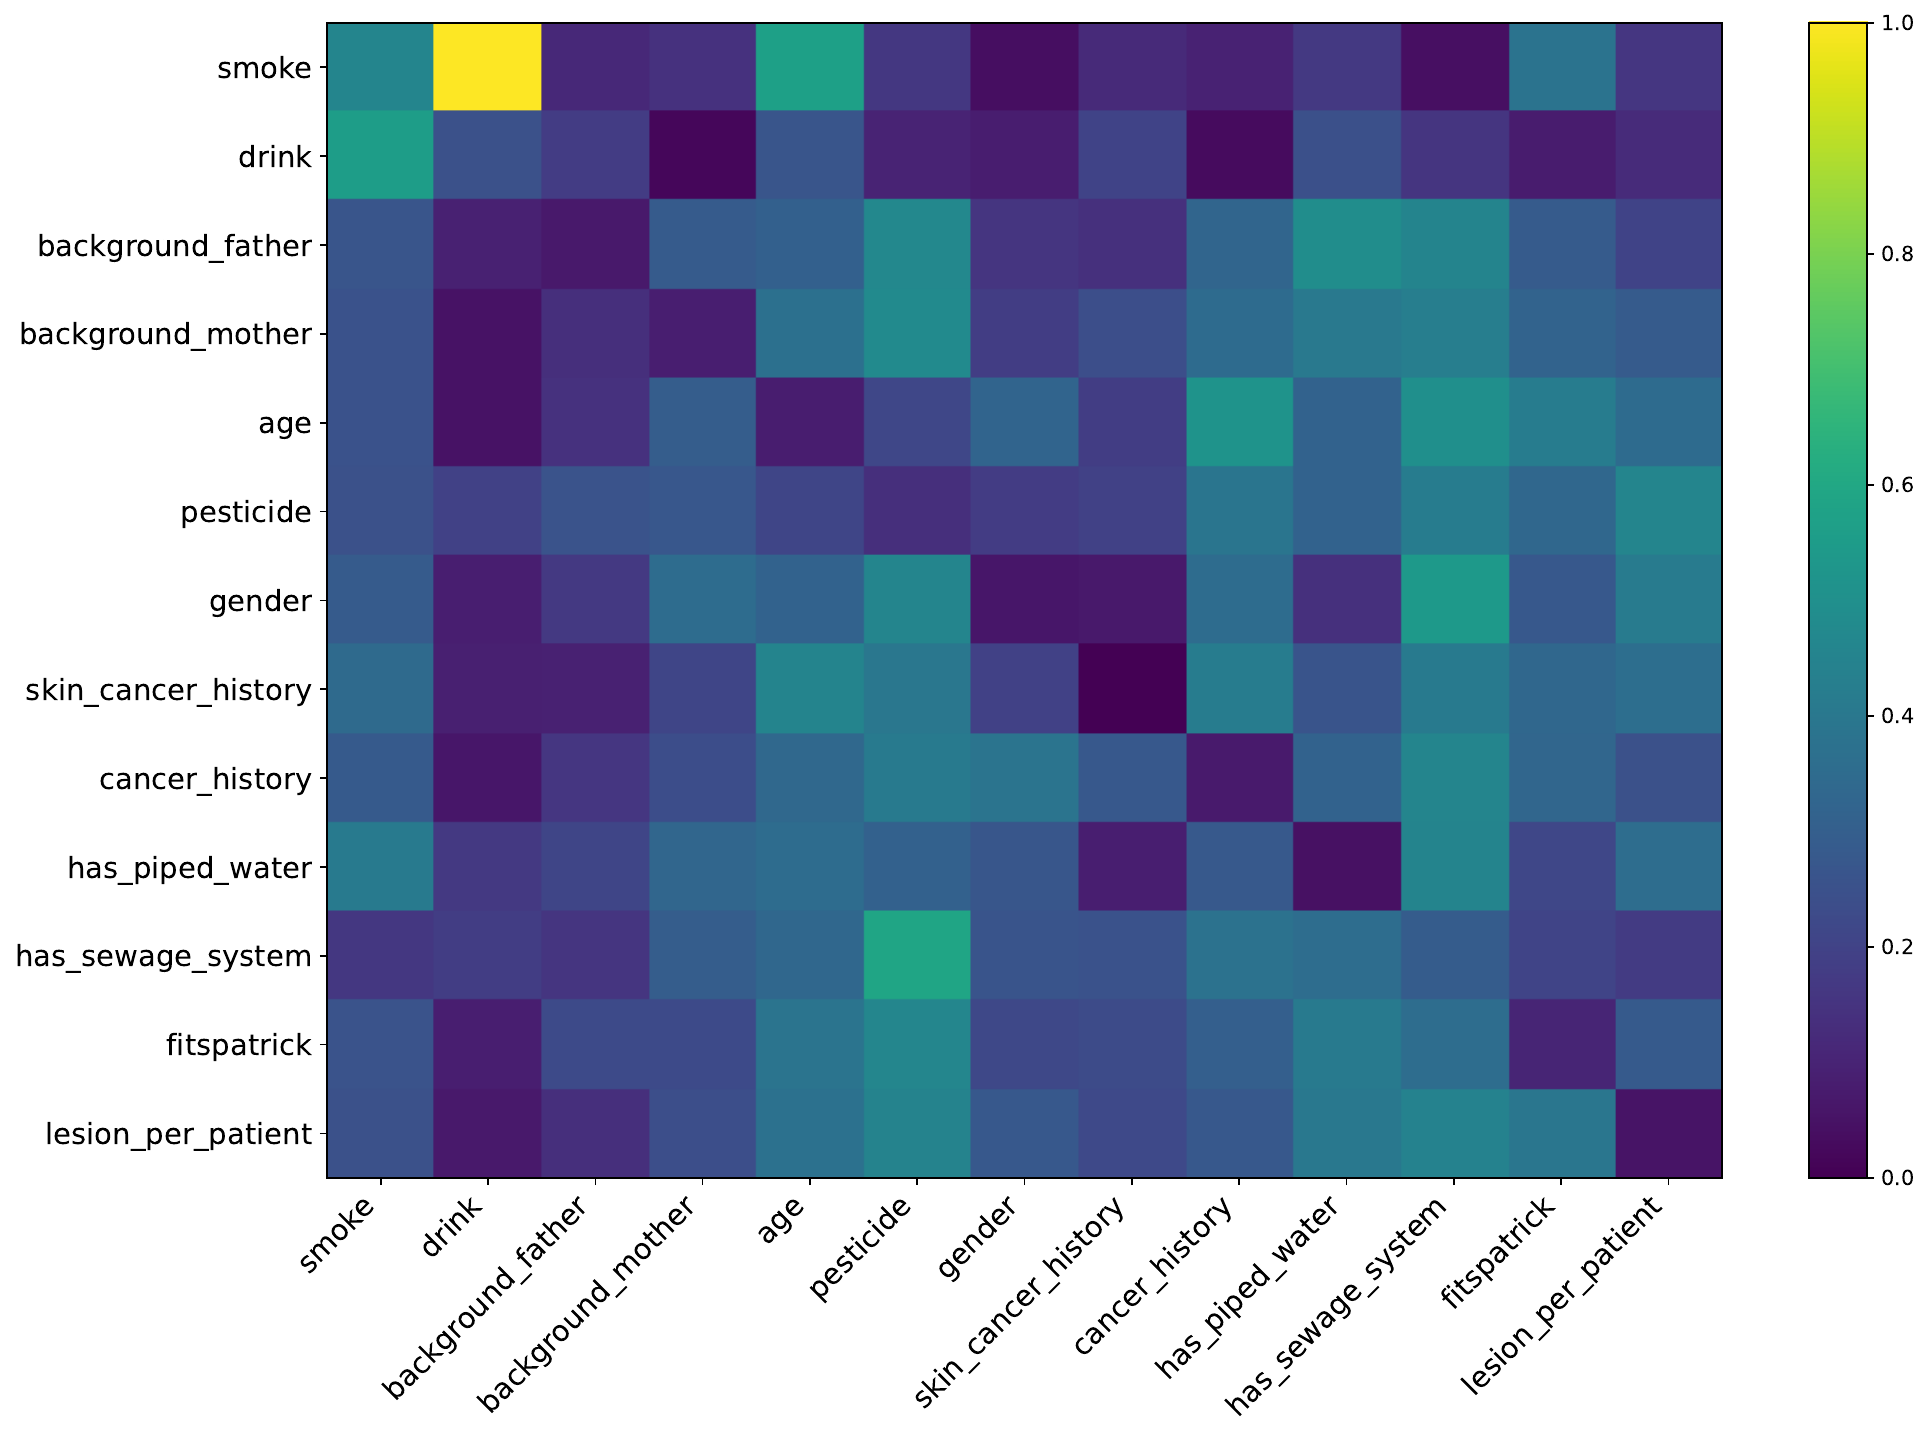} \\
    \end{tabular}

    \vspace{1em} % Vertical space between rows

    \begin{tabular}{cc} % Second row: two figures side-by-side
        Benign Lesion Features & Malignant Lesion Features \\ % Captions for the second row
        \includegraphics[width=0.5\textwidth]{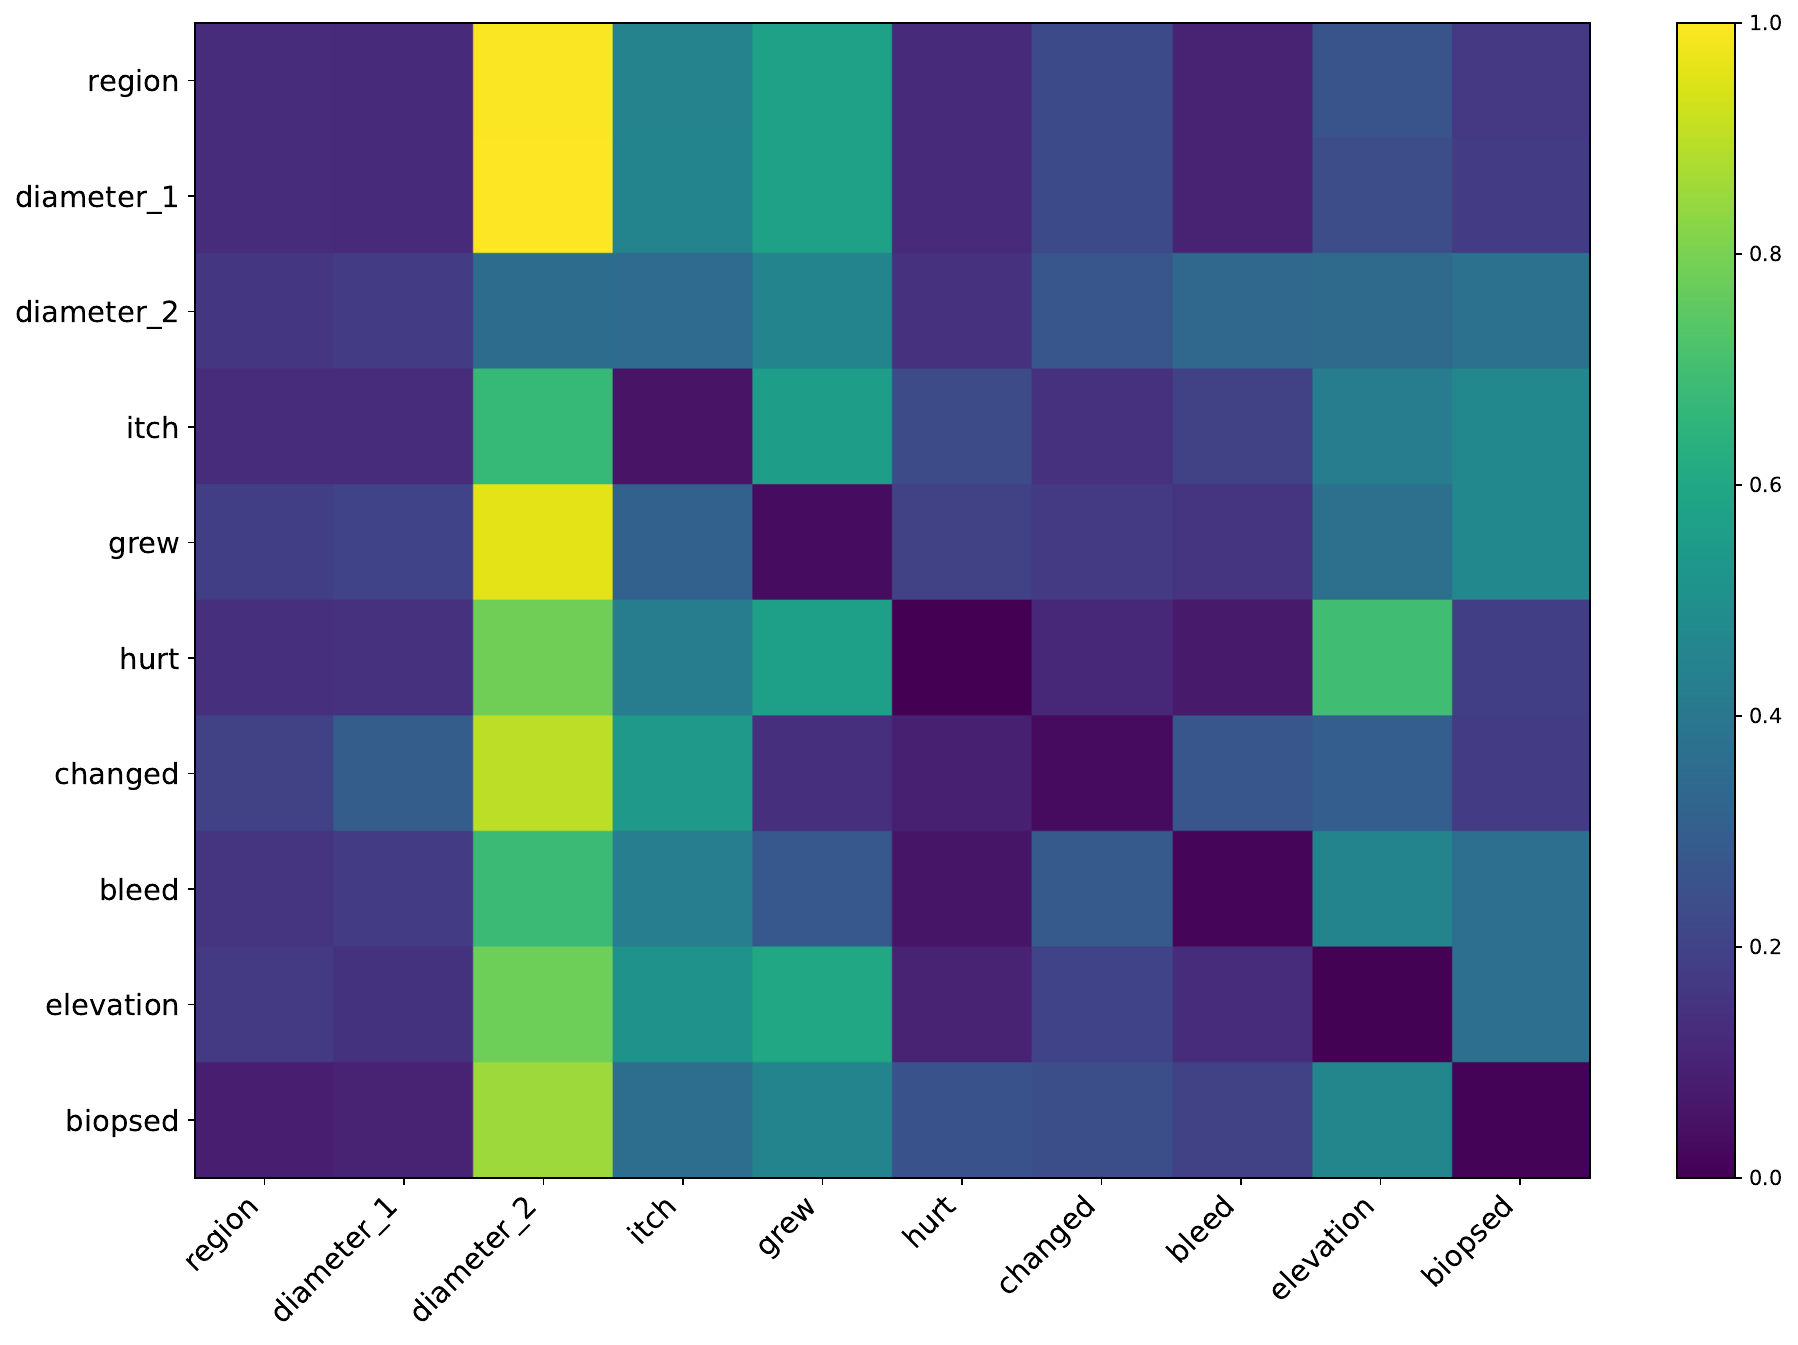} &
        \includegraphics[width=0.5\textwidth]{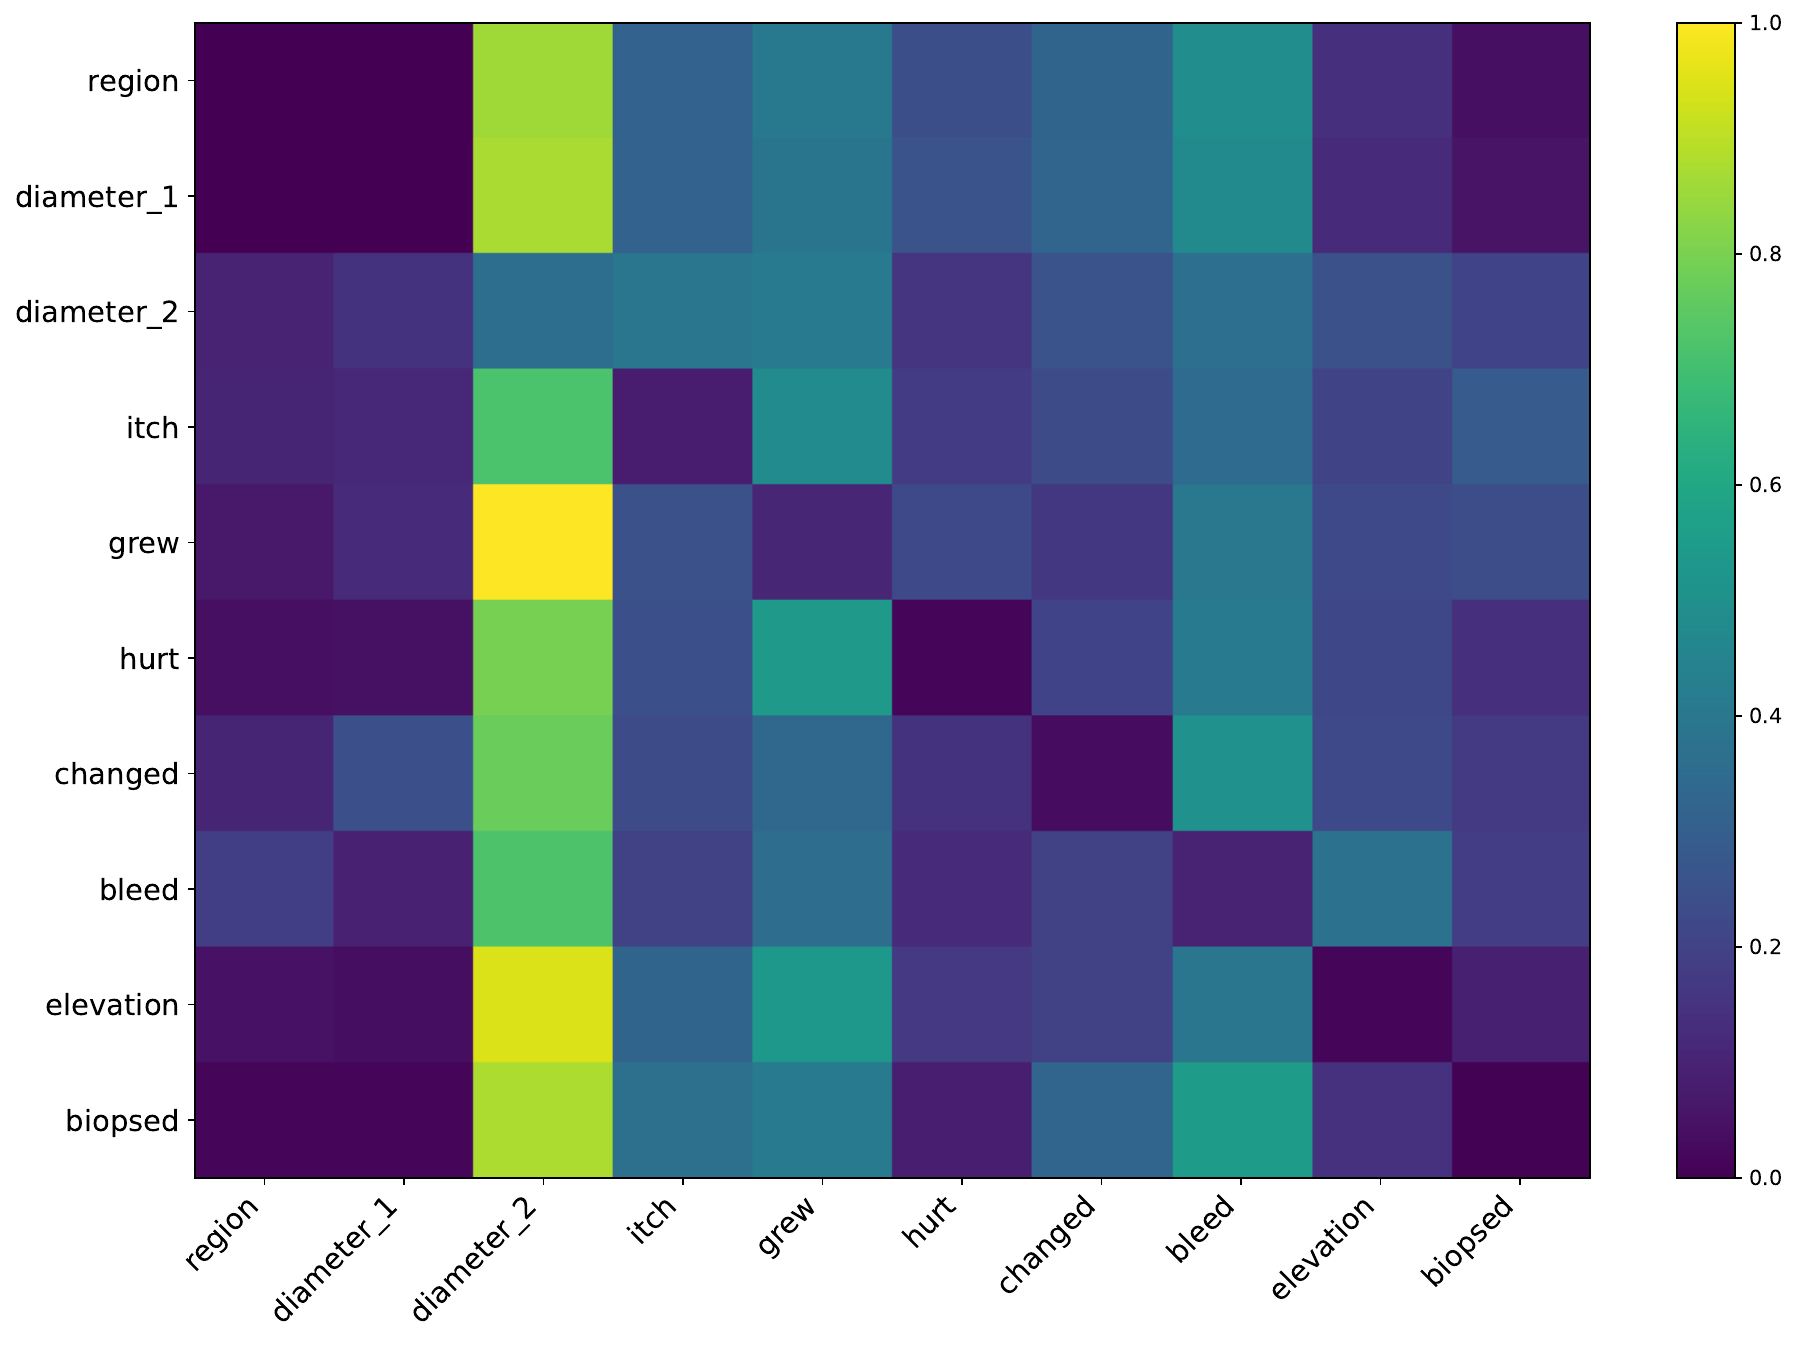} \\
    \end{tabular}

    \caption{Attention maps for the PAD-UFES-20 dataset.}
    \label{fig:padufes20_attention_maps}
\end{figure}

\begin{figure}[htb]
    \centering
    \begin{tabular}{c} % First row: single centered figure
        Clinical Features \\ % Caption for the first figure
        \includegraphics[width=0.5\textwidth]{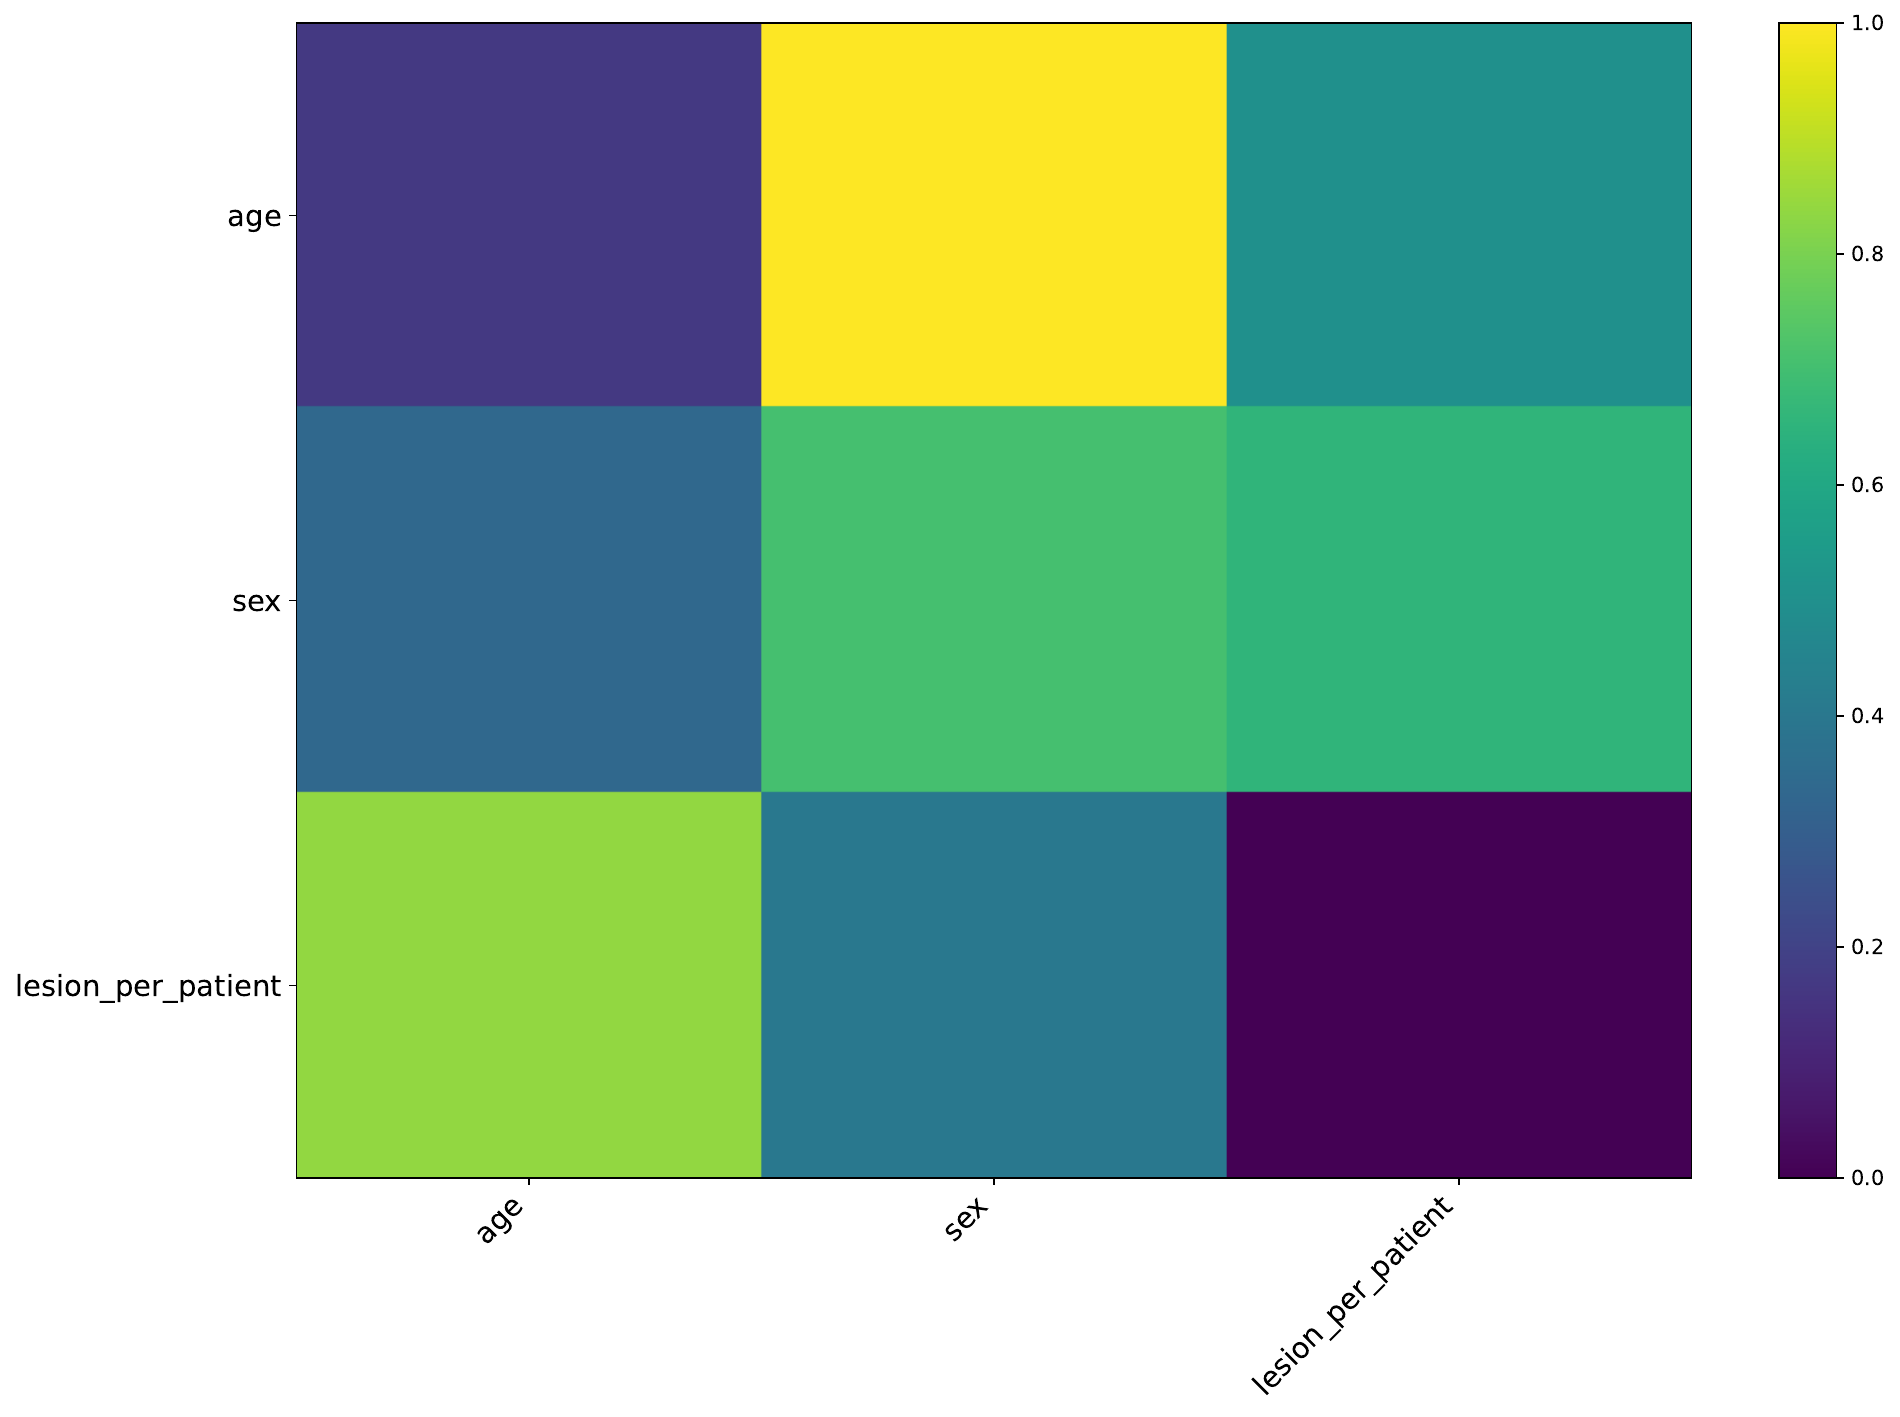} \\
    \end{tabular}

    \vspace{1em} % Vertical space between rows

    \begin{tabular}{cc} % Second row: two figures side-by-side
        Benign Lesion Features & Malignant Lesion Features \\ % Captions for the second row
        \includegraphics[width=0.5\textwidth]{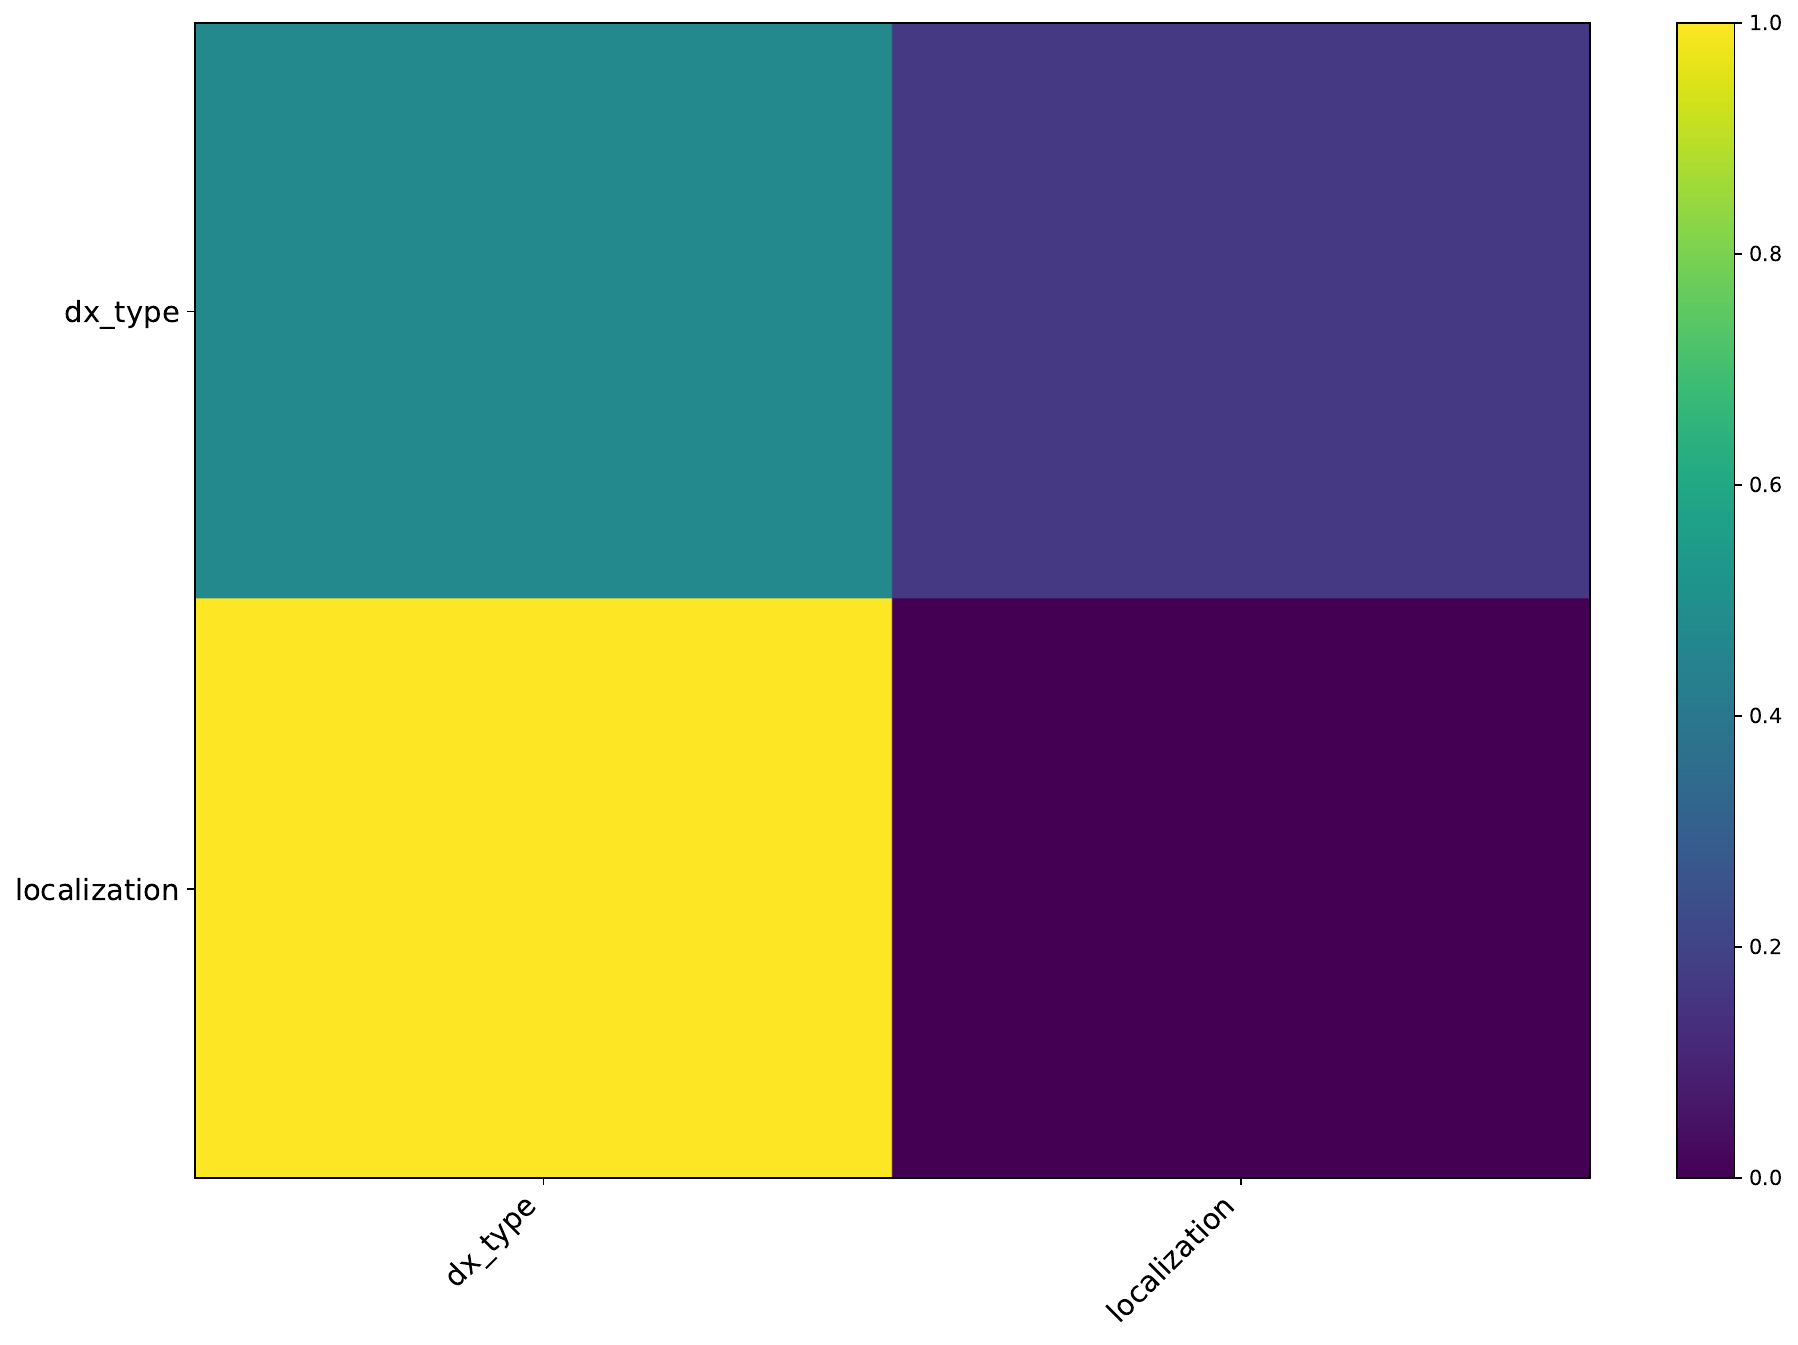} &
        \includegraphics[width=0.5\textwidth]{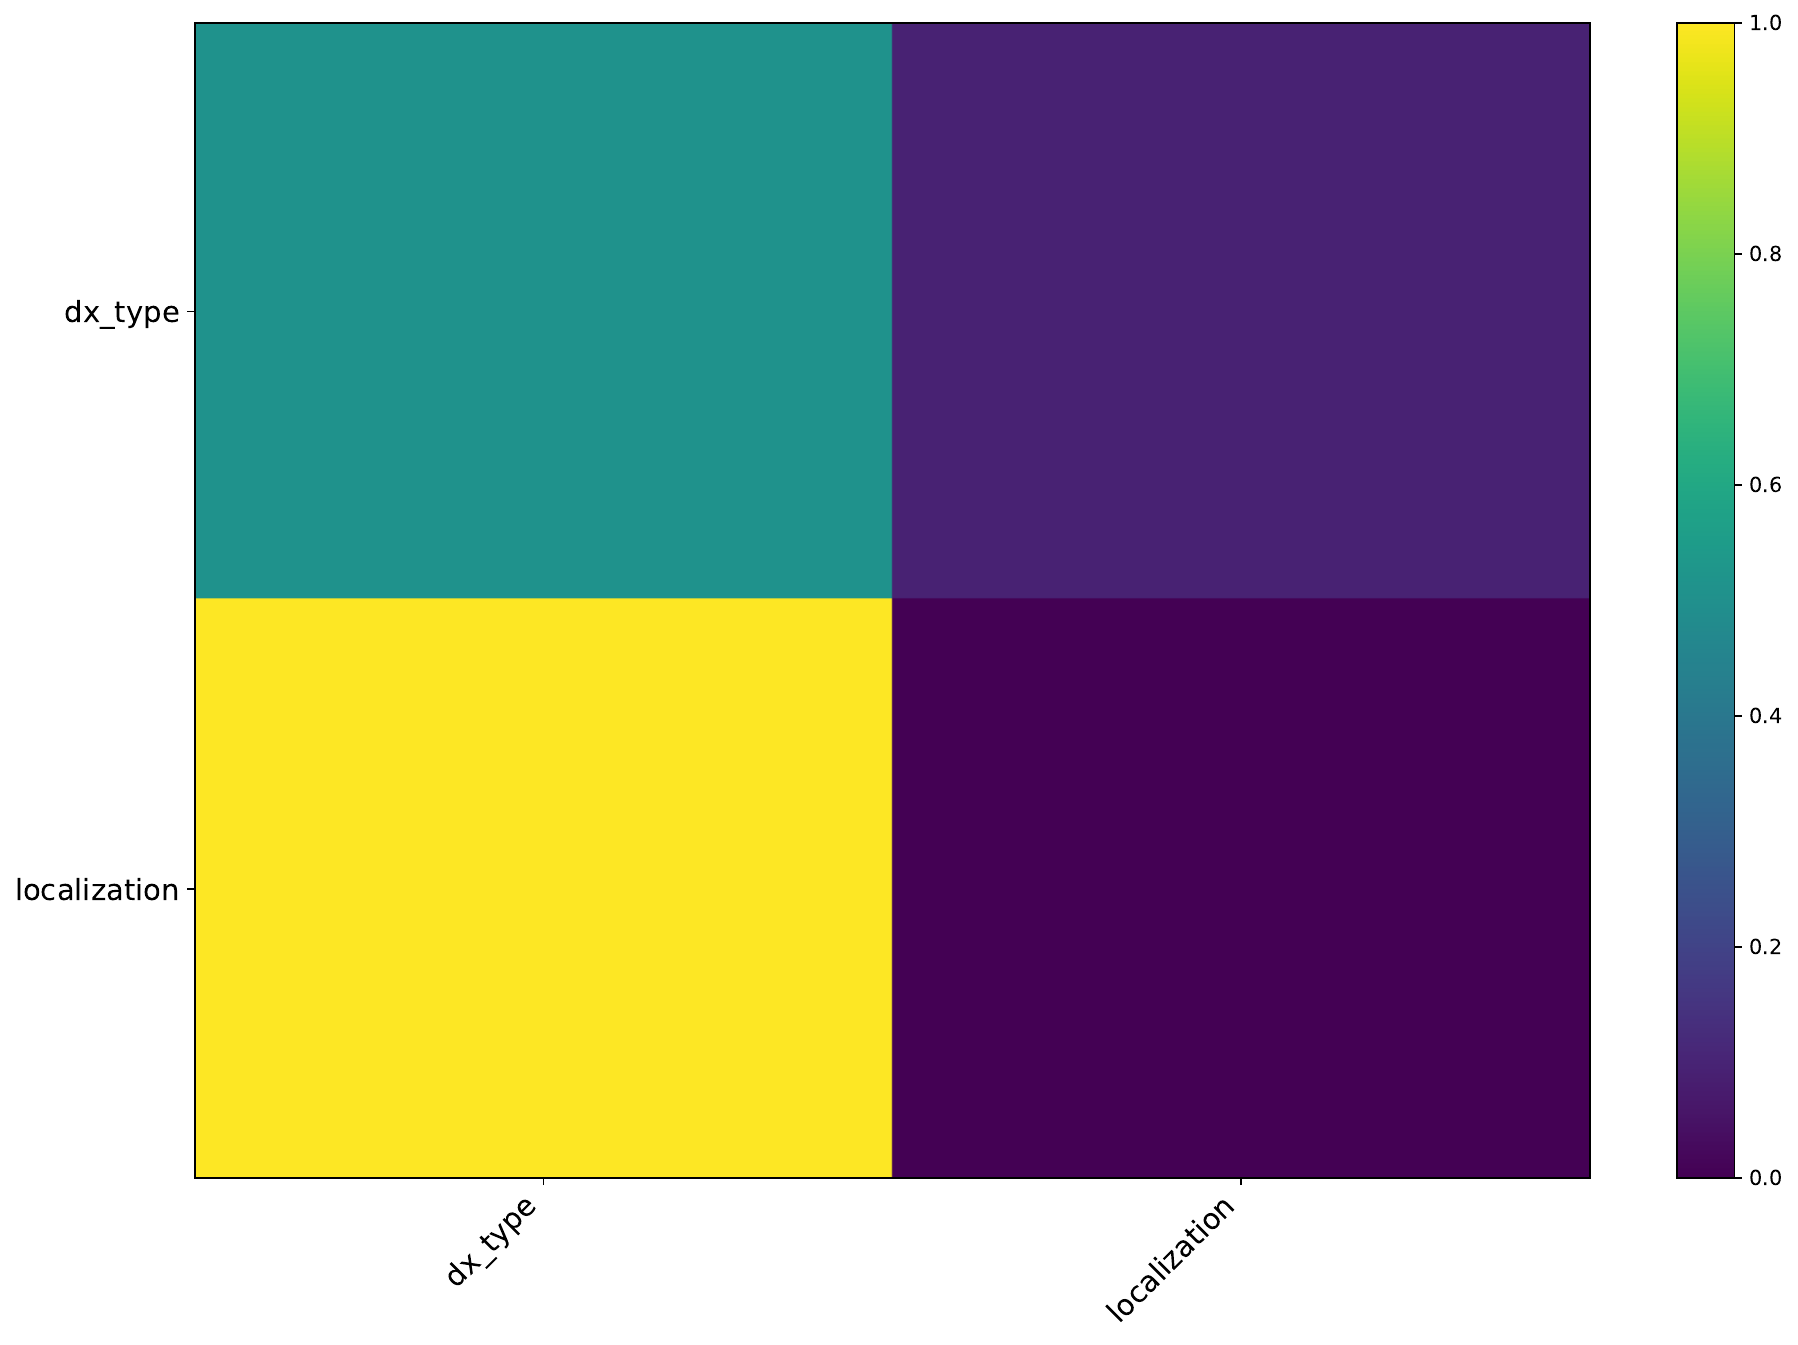} \\
    \end{tabular}

    \caption{Attention maps for the HAM10000 dataset.}
    \label{fig:ham10000_attention_maps}
\end{figure}

\begin{figure}[htb]
    \centering
    \begin{tabular}{c} % First row: single centered figure
        Clinical Features \\ % Caption for the first figure
        \includegraphics[width=0.5\textwidth]{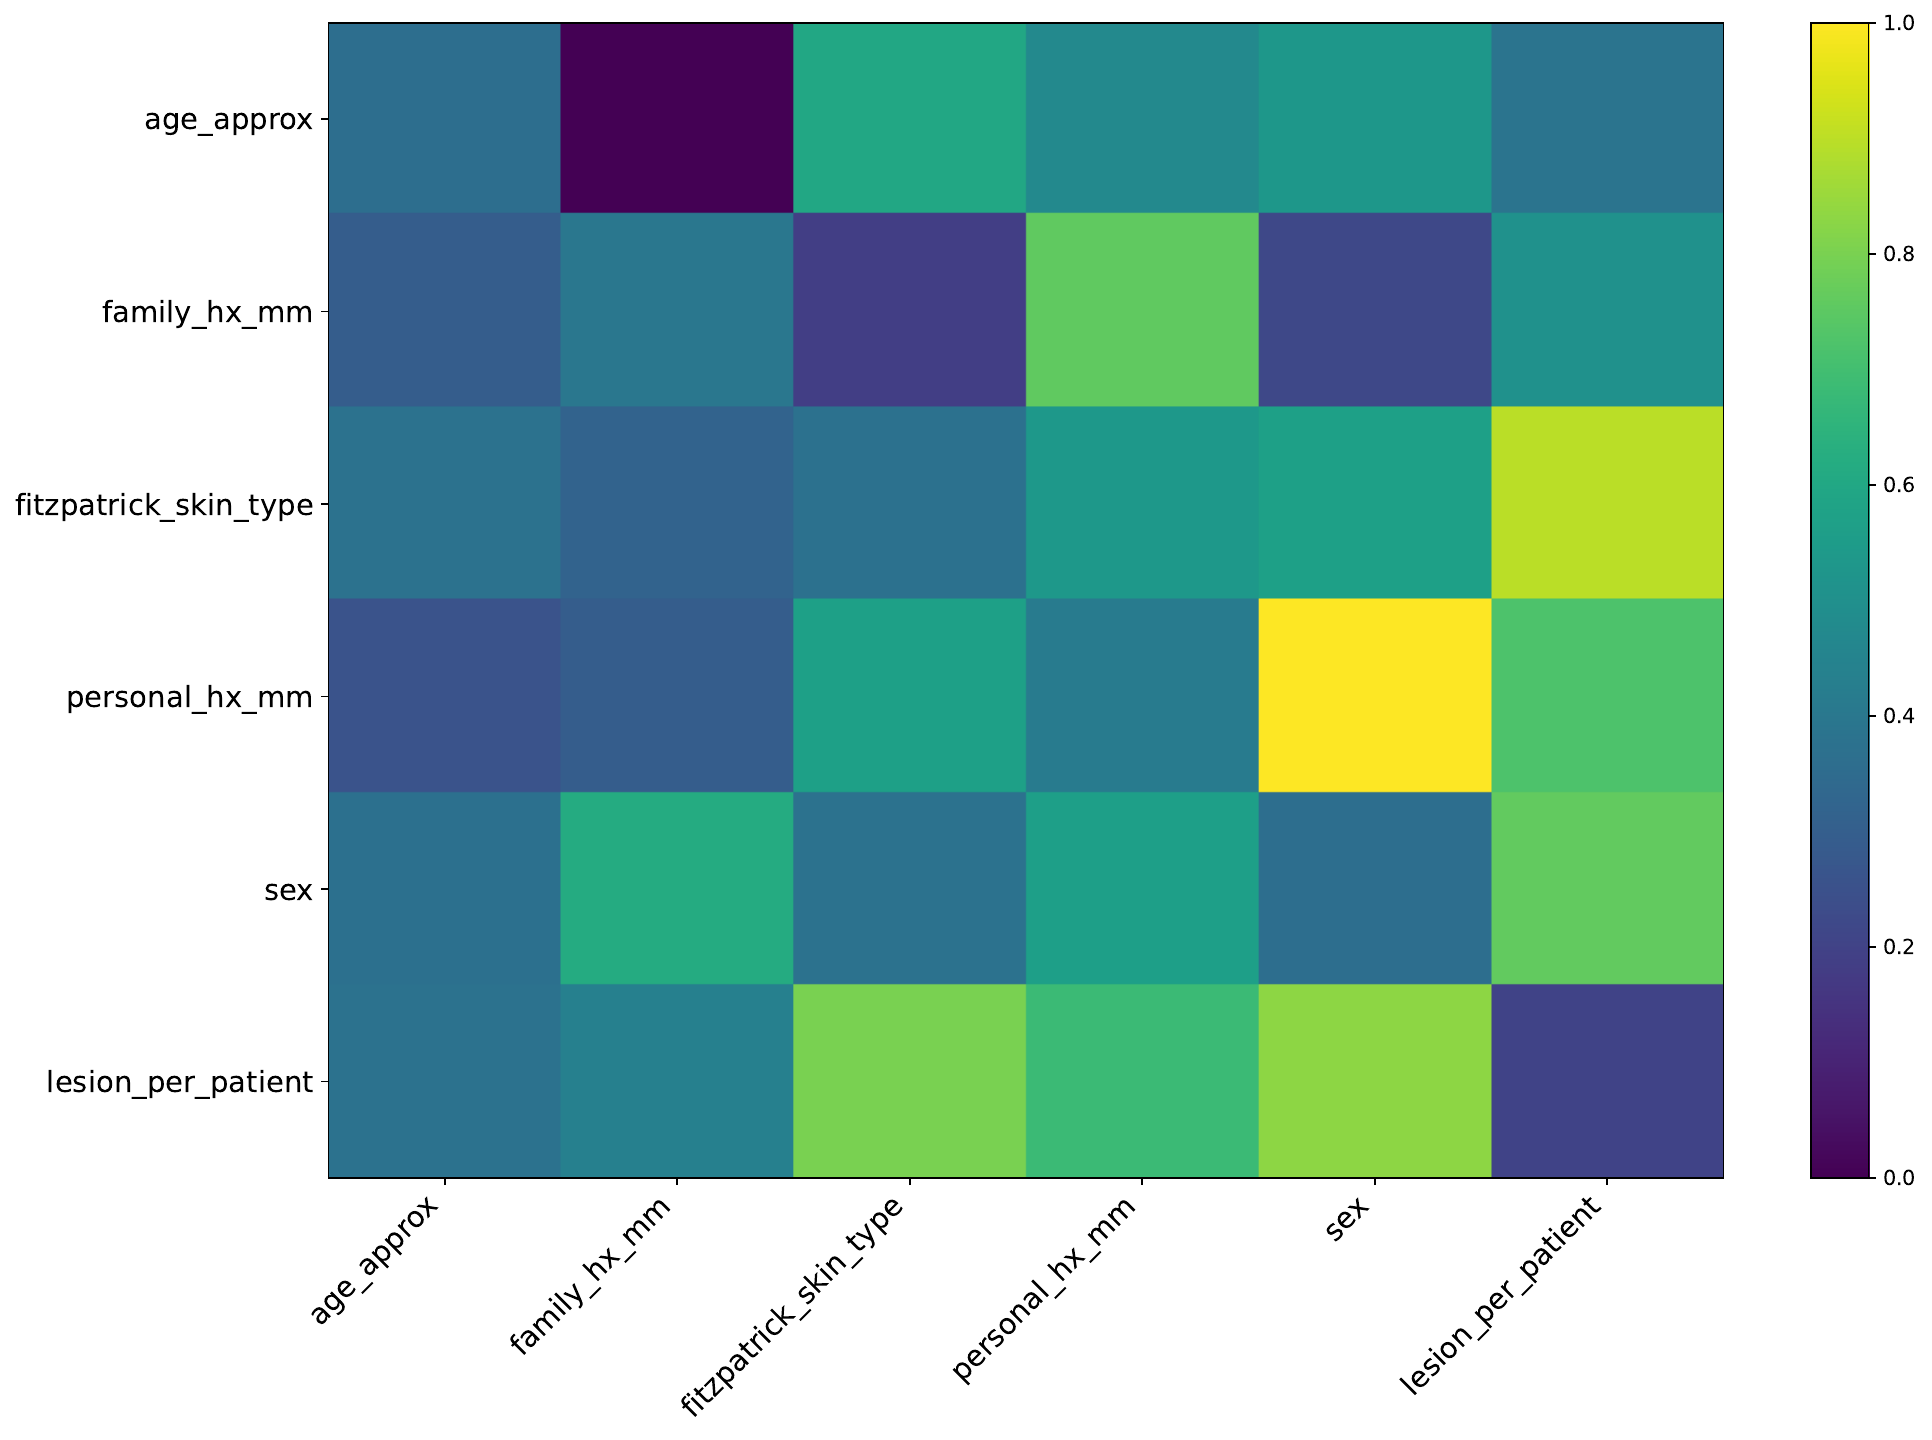} \\
    \end{tabular}

    \vspace{1em} % Vertical space between rows

    \begin{tabular}{cc} % Second row: two figures side-by-side
        Benign Lesion Features & Malignant Lesion Features \\ % Captions for the second row
        \includegraphics[width=0.5\textwidth]{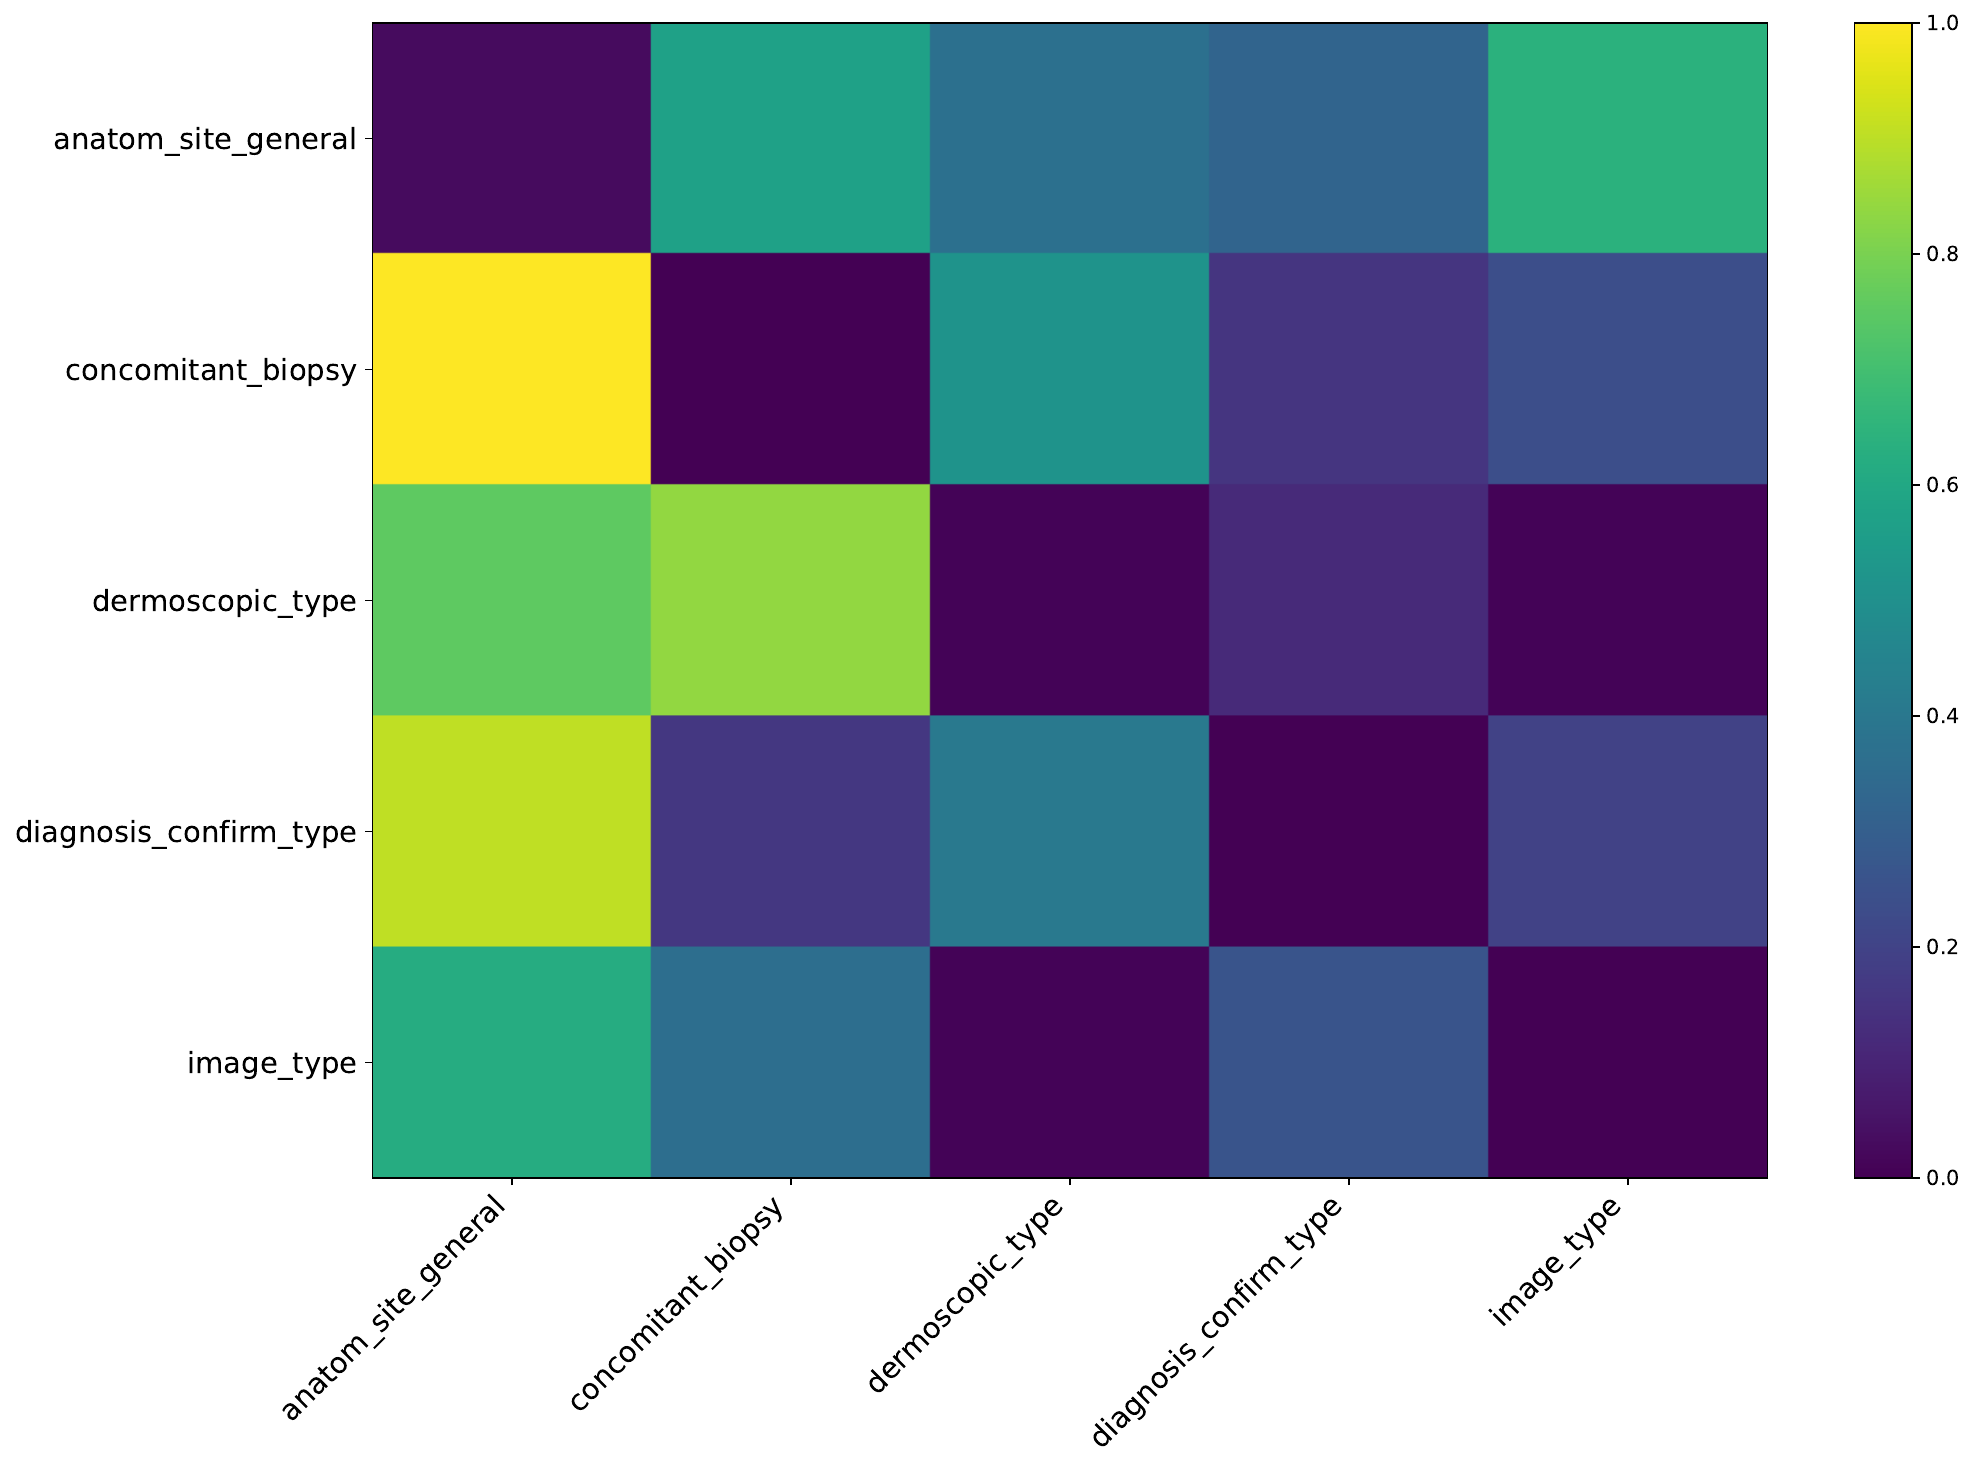} &
        \includegraphics[width=0.5\textwidth]{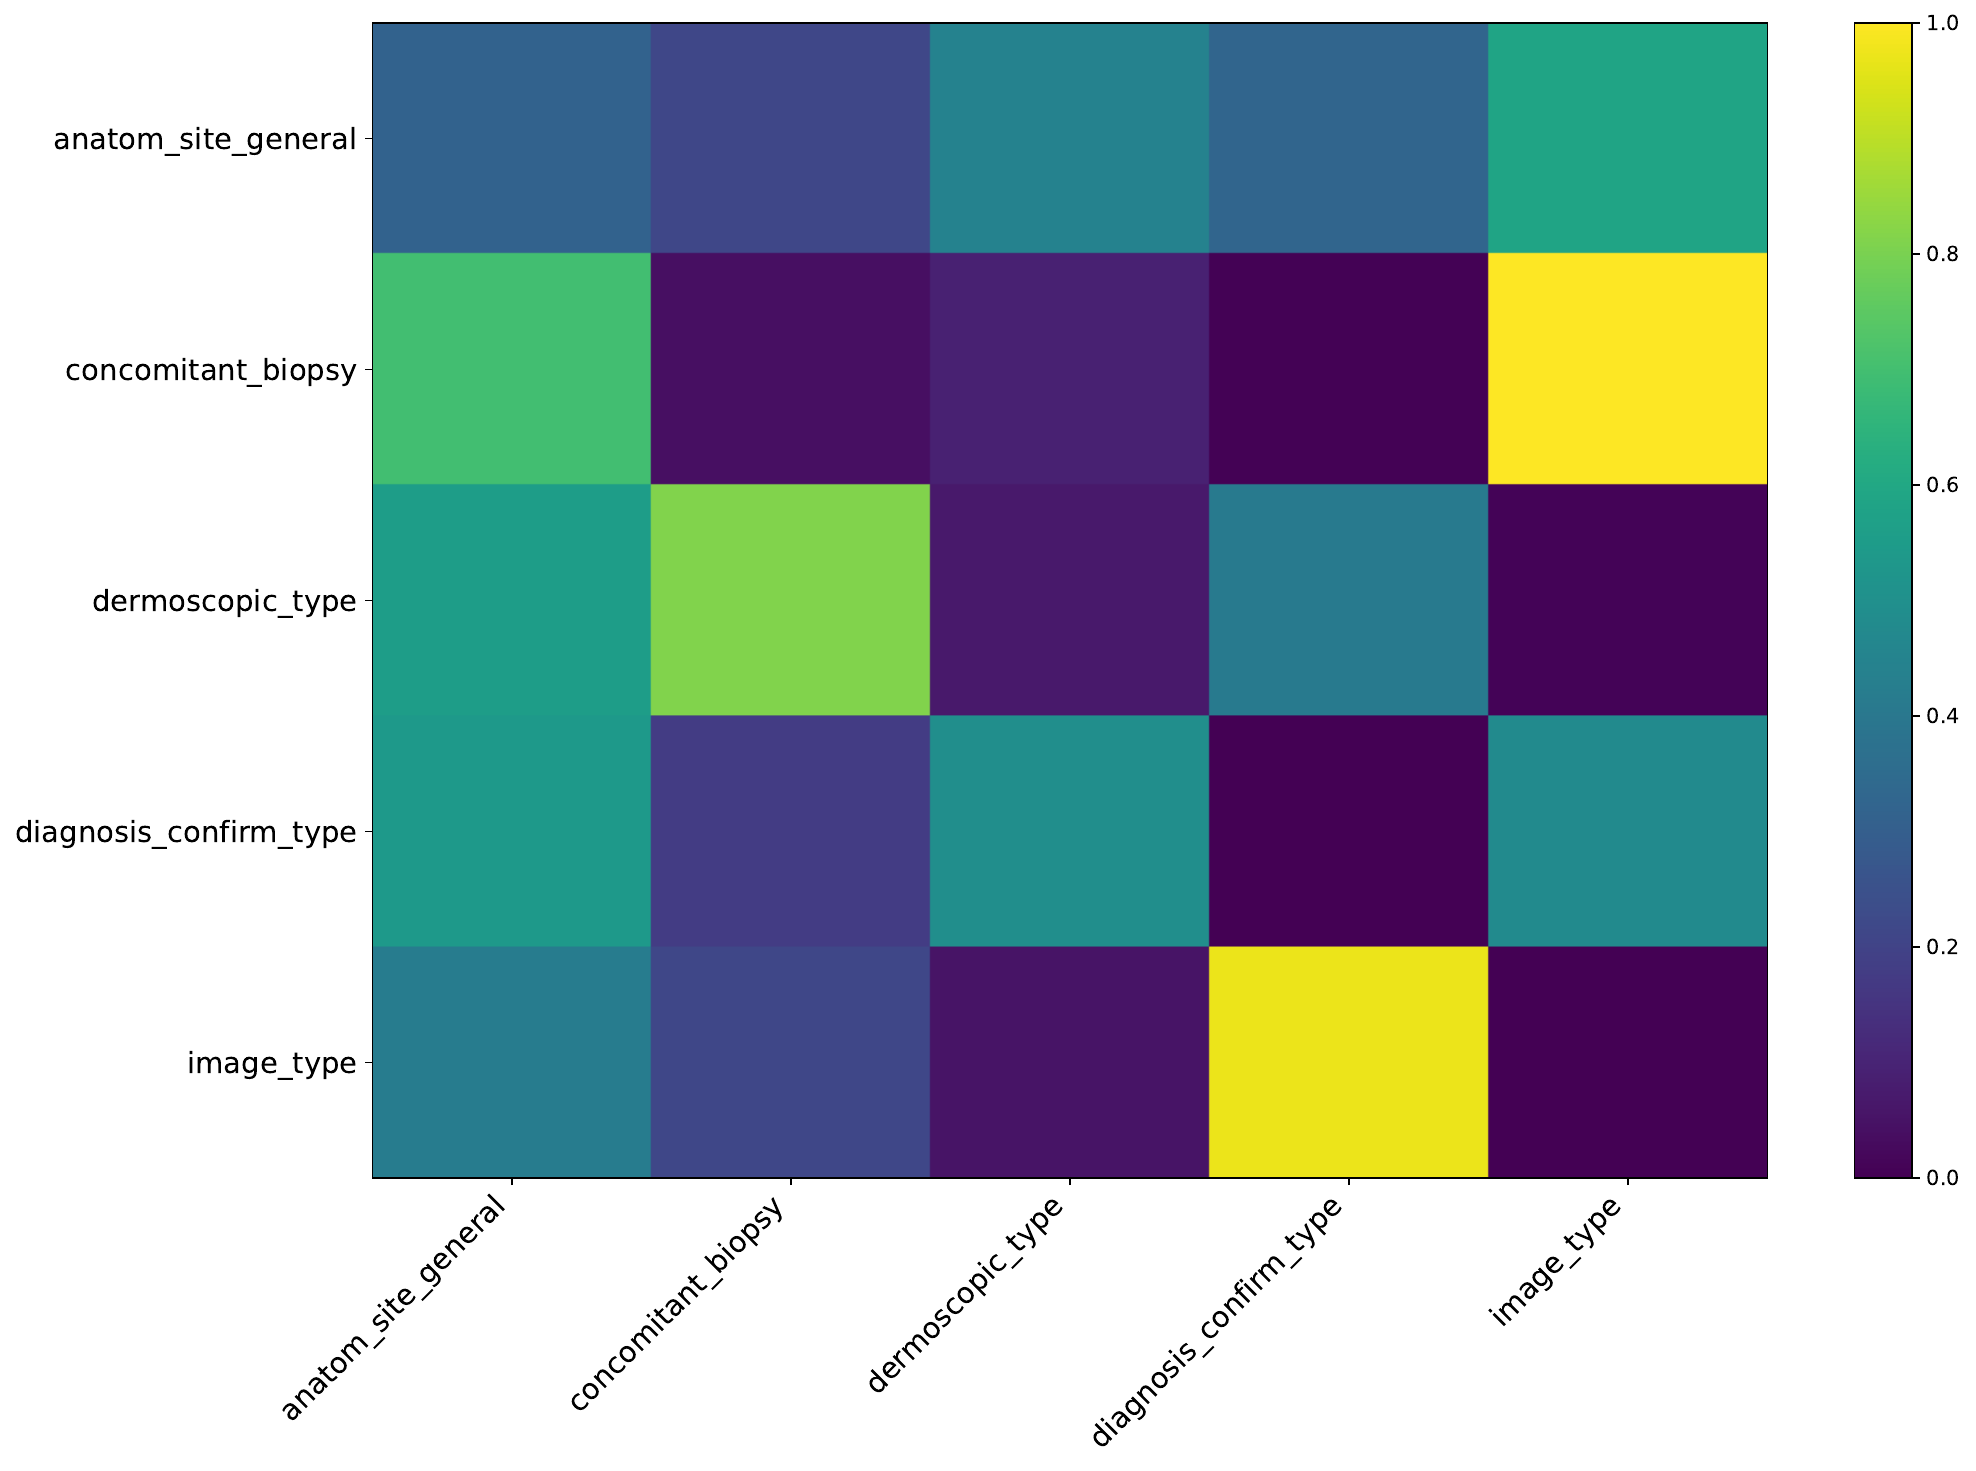} \\
    \end{tabular}

    \caption{Attention maps for the HIBA dataset.}
    \label{fig:hiba_attention_maps}
\end{figure}

\begin{figure}[htb]
    \centering
    \begin{tabular}{cc} % Second row: two figures side-by-side
        Benign Lesion Features & Malignant Lesion Features \\ % Captions for the second row
        \includegraphics[width=0.5\textwidth]{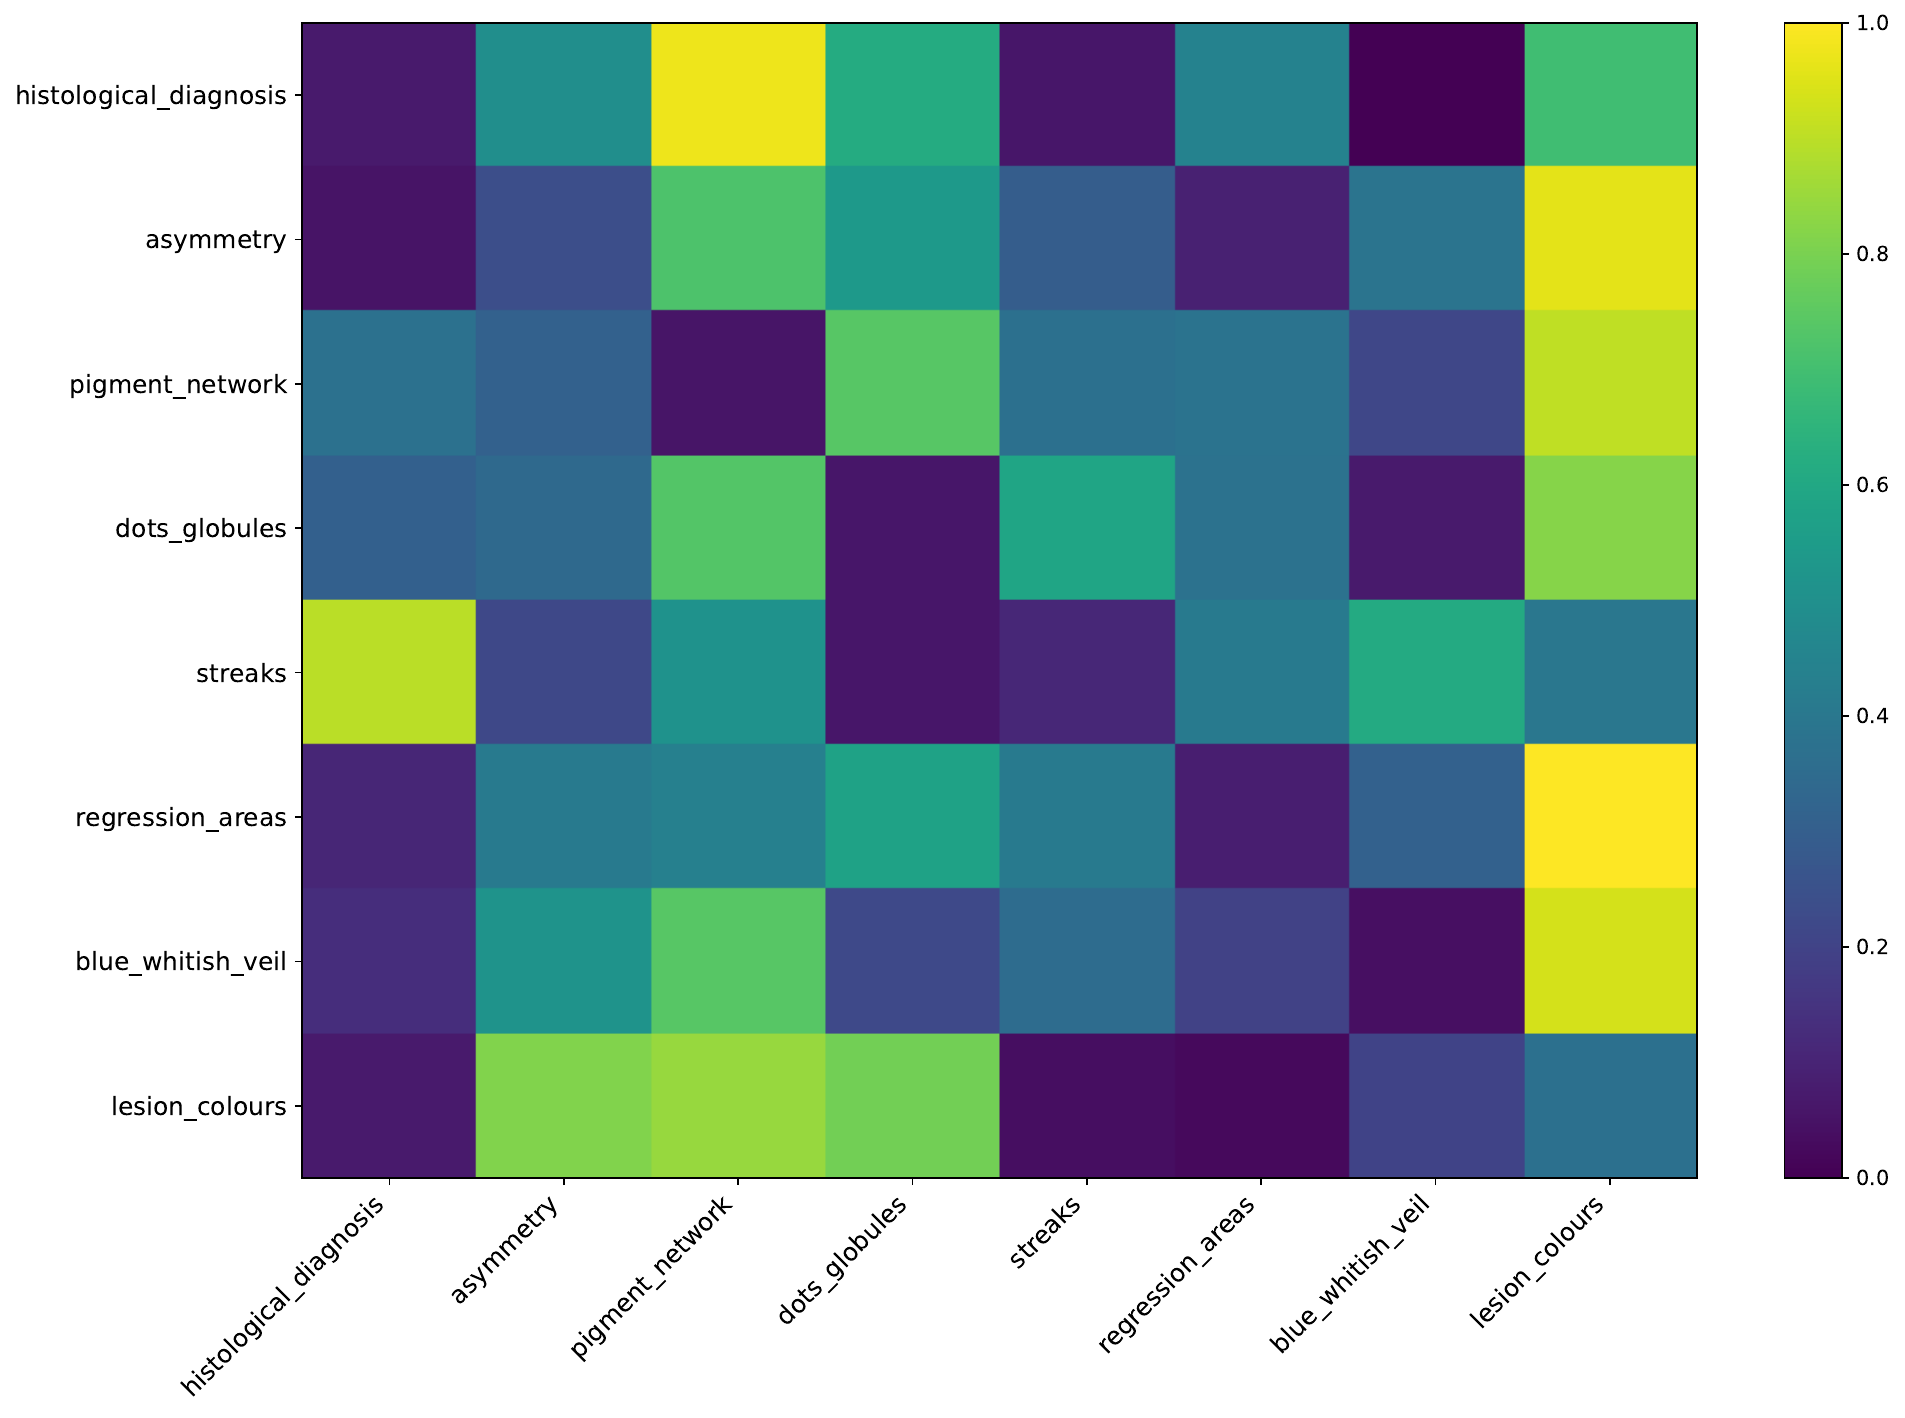} &
        \includegraphics[width=0.5\textwidth]{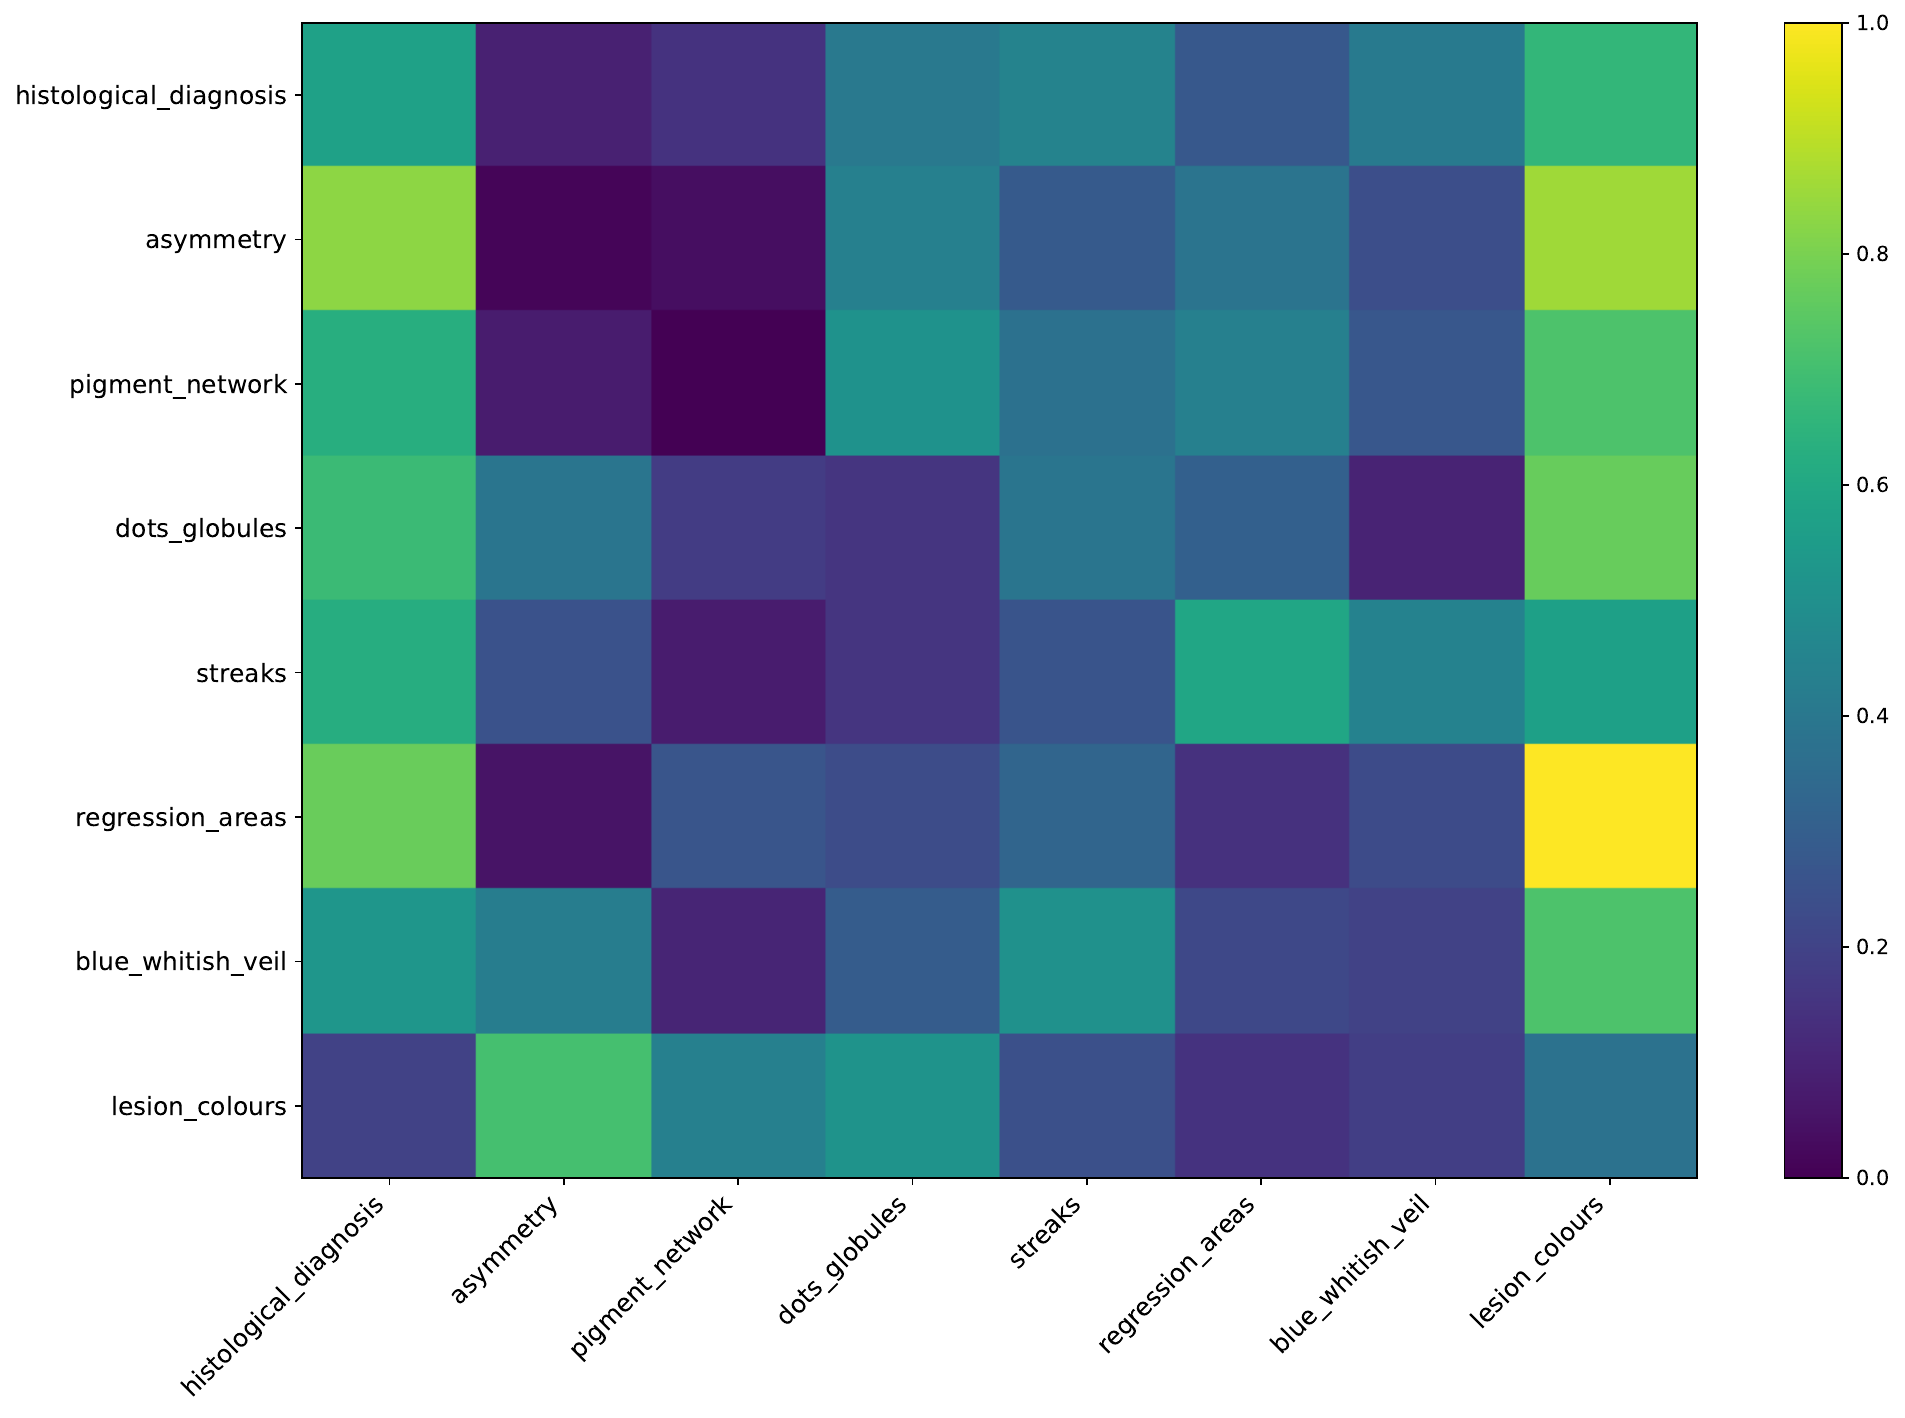} \\
    \end{tabular}
    \caption{Attention maps for the PH\textsuperscript{2} dataset.}
    \label{fig:ph2_attention_maps}
\end{figure}
